# Supplementary material for: GS-Playground: A High-Throughput Photorealistic Simulator for Vision-Informed Robot Learning
Source: arXiv:2604.25459 source file (2026-08-04)
Supplement: Supplementary file 1 [file 8_Appendix.tex]

\clearpage
\onecolumn

\appendices

\makeatletter
\def\@IEEEprocessthesectionargument#1{%
\@ifmtarg{#1}{%
\@IEEEappendixsavesection*{\appendixname~\thesectiondis}%
\addcontentsline{toc}{section}{\appendixname~\thesection}}{%
\@IEEEappendixsavesection*{\appendixname~\thesectiondis. #1}%
\addcontentsline{toc}{section}{\appendixname~\thesection. #1}}}
\makeatother

\newpage

\makeatletter
\global\@topnum 0
\makeatother

\addtocontents{toc}{\protect\setcounter{tocdepth}{3}}

\begin{center}
    \Huge \textbf{Appendix}
\end{center}

\etocsettocstyle{\section*{Table of Contents}}{}
\tableofcontents

\vspace{1em}
\hrule
\vspace{2em}

\makeatletter
\global\@topnum 0
\makeatother

\section{Physics}
\label{app:physics}

\subsection{Shaking Test}

To evaluate the stability and robustness of frictional contacts under dynamic perturbations, we conducted a "Shaking Test" using a Franka Panda arm. The robot grasps objects with different geometries—a cube, a ball, and a bottle—and executes aggressive random shaking motions. Each result aggregates 30 trials per object across three geometries. We compare the success rates of retaining the object across different physics engines at two simulation time steps: $dt=0.002s$ and $dt=0.01s$.

As shown in Table \ref{tab:franka_shaking} and Figure \ref{fig:shaking_scene}, \method demonstrates superior grasping robustness. The CPU backend achieves a 100\% success rate (90/90) across all object types and time steps, attributed to our velocity-impulse formulation and strict complementarity constraints which effectively prevent numerical drift and slippage. In contrast, MuJoCo variants (Euler, Implicit, and Implicit+Noslip) struggle significantly with this task, often dropping the object due to insufficient friction retention under high accelerations. IsaacSim and Genesis show better performance but still experience failures (60/90 success). Our GPU backend also maintains high stability, validating the effectiveness of our parallel solver design.

\begin{table}[t]
    \centering
    \caption{\small \textbf{Grasping robustness under external disturbances}. Success rates for a Franka Panda holding various geometries (cube, ball, bottle) under random shaking. A trial is successful if the object is retained for the entire evaluation horizon. 
    }
    \scalebox{1}{
        \begin{tabular}{lcc}
            \toprule
            \textbf{Engine} & \textbf{dt=0.002s (success)} & \textbf{dt=0.01s (success)} \\
            \midrule
            MuJoCo (Euler) & 0/90 & 0/90 \\
            MuJoCo (Implicit) & 0/90 & 0/90 \\
            MuJoCo (Implicit+Noslip) & 4/90 & 0/90 \\
            MJWarp & 0/90 & 10/90 \\
            IsaacSim & 60/90 & 60/90 \\
            Genesis & 60/90 & 60/90 \\
            Ours (CPU) & \textbf{90/90} & \textbf{90/90} \\
            Ours (GPU) & \textbf{90/90} & \textbf{74/90} \\
            \bottomrule
        \end{tabular}
    }
    \label{tab:franka_shaking}
\end{table}

\begin{figure}[h!]
\centering
\includegraphics[width=0.5\linewidth]{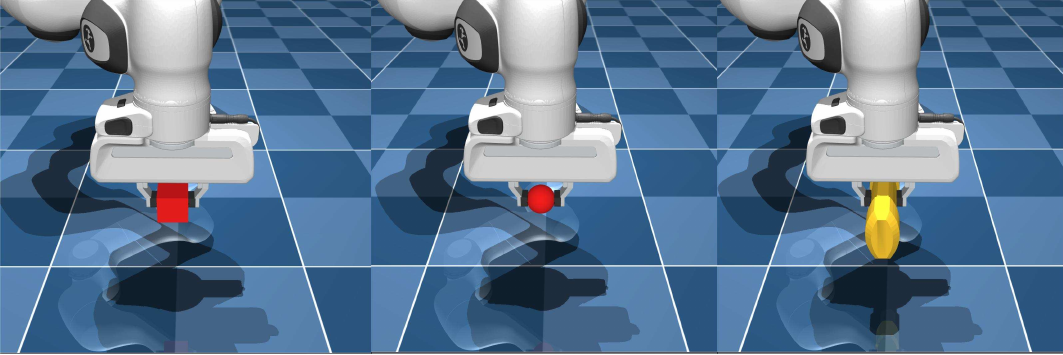}
\caption{\textbf{Shaking Test Scene}: A Franka Panda robot grasps various objects (a cube, a ball, and a bottle) while being subjected to random shaking motions. This setup is used to evaluate the grasping robustness of different simulation methods under dynamic perturbations.}
\vspace{-4mm}
\label{fig:shaking_scene}
\end{figure}

\begin{figure}[t]
    \centering
    \includegraphics[width=0.6\linewidth]{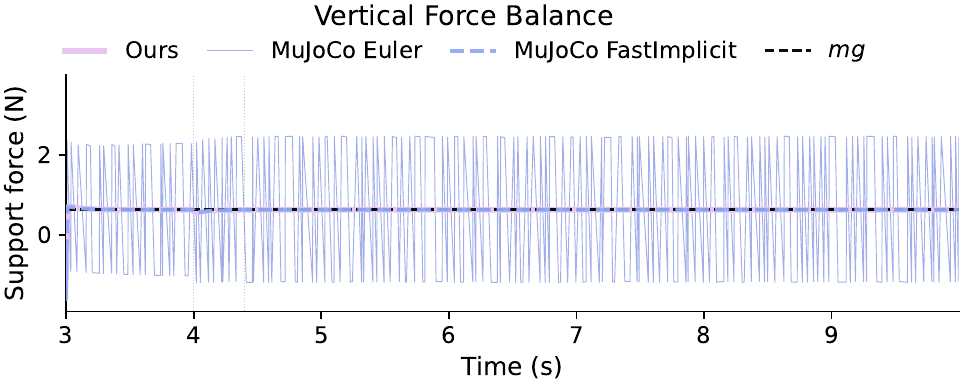}
    \caption{\textbf{Vertical force balance in a Panda grasp.}
    The plot compares the vertical contact support force $F_z$ with the theoretical object weight $mg$ during lift, settling, and hold. MuJoCo Euler exhibits large oscillatory contact forces, while \method and MuJoCo FastImplicit remain close to the force-balance target.}
    \label{fig:grasp_force_balance}
\end{figure}

\begin{table}[t]
    \centering
    \caption{\textbf{Hold-stage vertical force-balance error.}
    Mean absolute error between the measured vertical support force $F_z$ and the object weight $mg$ for the hold phase in Fig.~\ref{fig:grasp_force_balance}.}
    \label{tab:grasp_force_balance_error}
    \setlength{\tabcolsep}{5pt}
    \scalebox{0.95}{
        \begin{tabular}{lc}
            \toprule
            \textbf{Engine} & \textbf{Mean $\lvert F_z - mg \rvert$ (mN)} \\
            \midrule
            Ours & \textbf{0.039} \\
            MuJoCo FastImplicit & 0.039 \\
            MuJoCo Euler & 1740.233 \\
            \bottomrule
        \end{tabular}
    }
\end{table}

\begin{table}[t]
    \centering
    \caption{\small \textbf{Critical-friction hold test}. Each trial starts from the initialized Panda grasp hold state and runs for 5\,s with friction coefficient $\mu=\alpha\mu_{\mathrm{crit}}$. Here $\mu_{\mathrm{crit}}=mg/N=0.0902$, with $N\approx6.962$\,N and $mg=0.6278$\,N. Numeric entries report the first drop time in seconds; $\checkmark$ indicates the object remained held for the full trial. $\dagger$ marks an outcome that violates the theoretical hold/drop expectation.}
    \setlength{\tabcolsep}{3pt}
    \scalebox{0.95}{
        \begin{tabular}{lccccc}
            \toprule
            \textbf{Engine} & \textbf{0.90x} & \textbf{0.98x} & \textbf{1.00x} & \textbf{1.02x} & \textbf{1.10x} \\
            \midrule
            Theory & Drop & Drop & Hold & Hold & Hold \\
            \midrule
            \method & 0.10 & 0.25 & \textbf{$\checkmark$} & \textbf{$\checkmark$} & \textbf{$\checkmark$} \\
            MuJoCo Euler & 0.07 & 0.08 & 0.08$^\dagger$ & 0.08$^\dagger$ & 0.07$^\dagger$ \\
            MuJoCo FastImplicit & 0.10 & 0.21 & 1.23$^\dagger$ & 2.00$^\dagger$ & 2.70$^\dagger$ \\
            \bottomrule
        \end{tabular}
    }
    \label{tab:critical_friction_hold}
\end{table}

\subsection{Quantitative Grasp Force Stability}
\label{app:quantitative_grasp_force_stability}

\begin{figure}
    \centering
    \includegraphics[width=0.5\linewidth]{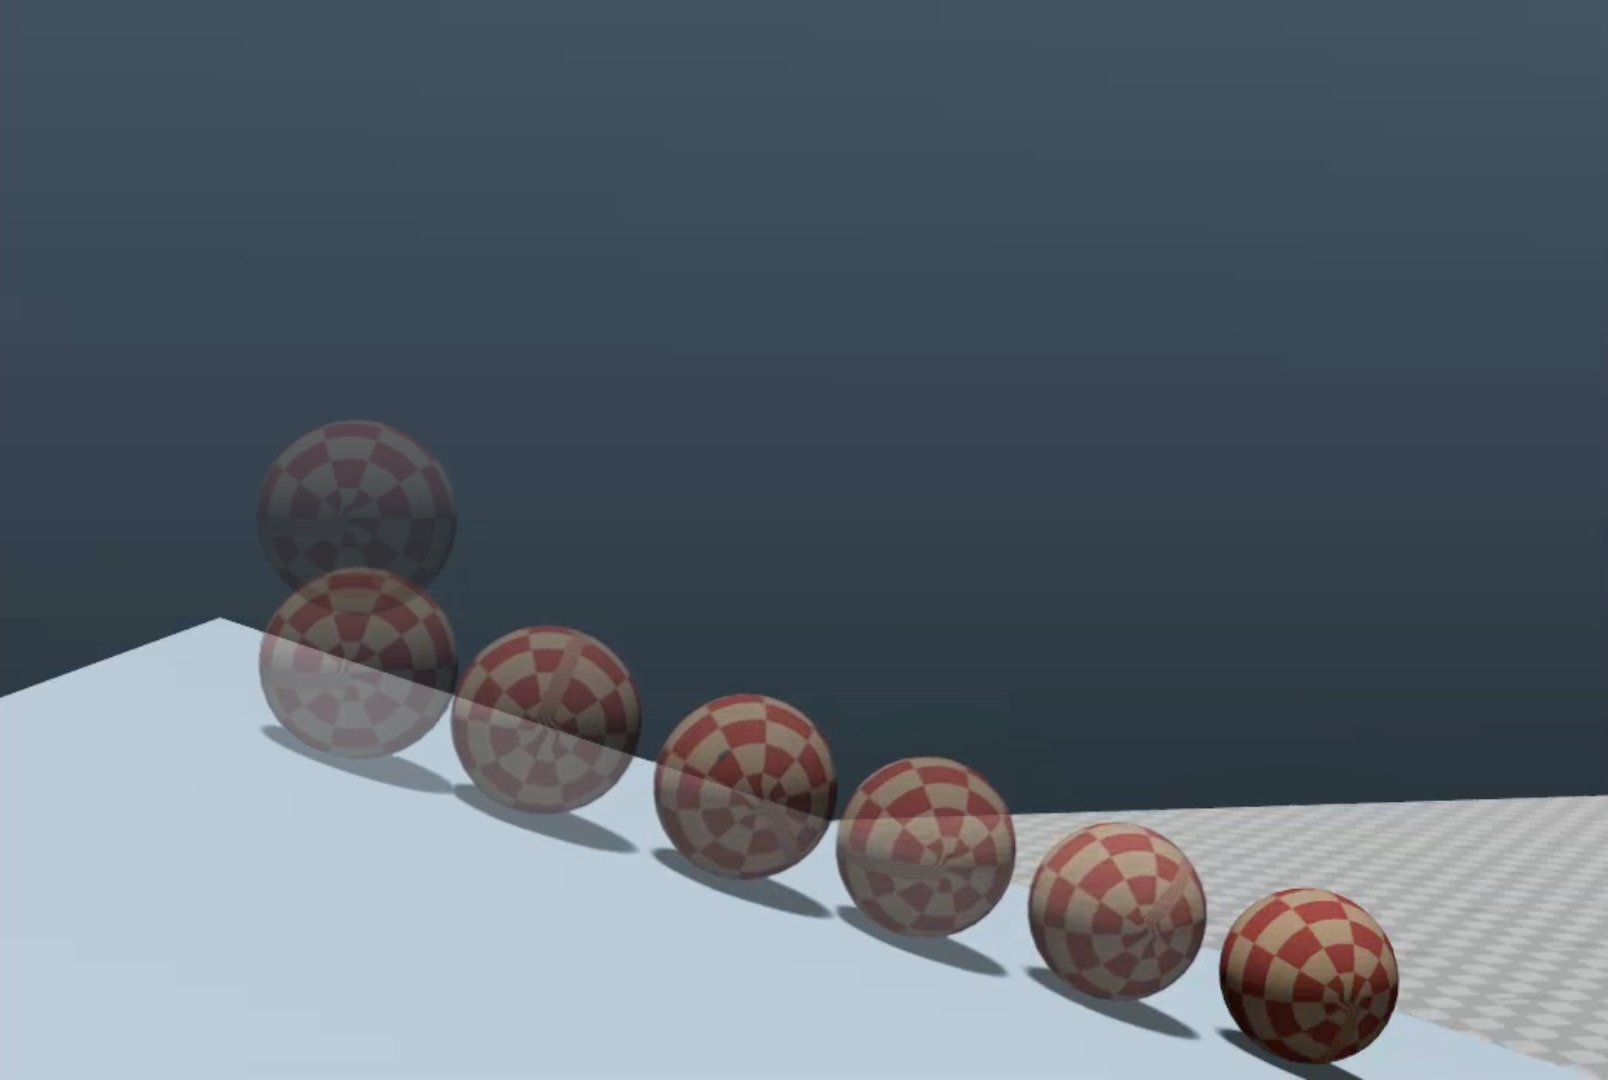}
    \caption{\textbf{Ball falling Scene:} A ball falls onto the inclined plane.}
    \label{fig:ball_falling_scene}
\end{figure}

\begin{figure}[t]
    \centering
    \includegraphics[width=0.5\linewidth]{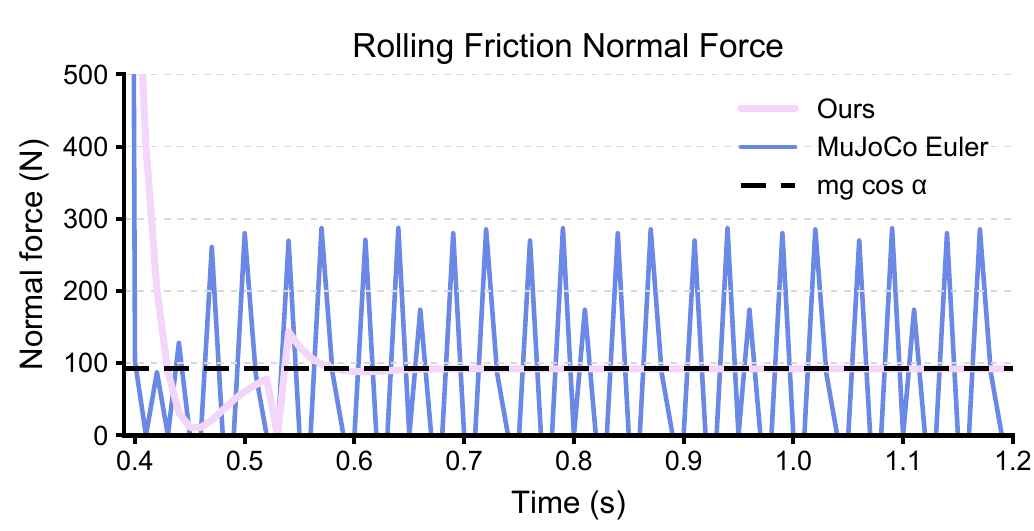}
    \caption{\textbf{Rolling friction normal force.}
    This diagram compares the normal force acting on the small ball after it contacts the inclined plane.}
    \label{fig:rolling_friction_comparison}
\end{figure}

While the shaking test evaluates task-level robustness under dynamic disturbances, it does not isolate the contact-force behavior behind a successful grasp. We therefore further examine a quasi-static hold setting where the primary question is not whether the object is retained, but whether the simulated contact forces remain physically consistent and stable.

\noindent\textbf{Vertical force balance.}
To evaluate contact stability in a quasi-static manipulation setting, we conduct a grasp hold test with a Franka Panda gripper lifting and holding a rigid cube. The robot follows the same staged trajectory for all simulators: approaching the object, closing the gripper, lifting the cube, settling after the lift, and finally maintaining a fixed hold. We compare \method against MuJoCo Euler and MuJoCo FastImplicit under the same model, control schedule, timestep, and contact-sensor layout.

The test measures whether the finger contacts provide a physically consistent vertical support force after the object leaves the table. At each simulation step, we aggregate the tangential contact forces reported by the left and right finger sensors and extract their vertical component $F_z$. During the hold phase, the expected support force is the object's weight $mg$; therefore, a stable contact solve should keep $F_z$ close to $mg$ while avoiding high-frequency oscillations. Table~\ref{tab:grasp_force_balance_error} summarizes this condition with the hold-stage mean absolute force-balance error, reported in millinewtons.

The results show that integrator choice has a strong effect on MuJoCo's contact response. Although all methods retain the object through the final hold state, MuJoCo Euler produces pronounced oscillations in the vertical support force and high hold-stage force jitter. MuJoCo FastImplicit largely suppresses this oscillation and reaches a force-balance accuracy similar to \method. In contrast, \method achieves this stable balance in its default configuration: during the hold phase, its object-height variation is $0.045$\,mm, compared with $0.230$\,mm for MuJoCo Euler and $0.190$\,mm for MuJoCo FastImplicit. This experiment therefore isolates a contact-rich manipulation regime where stable force balance, rather than binary grasp success, is the primary measurement target.

\smallskip
\noindent\textbf{Critical-friction hold.}
We further test whether the same hold state remains stable when the sliding friction coefficient is set near the theoretical limit. After a warm-up hold phase, we estimate the total normal gripping force $N$ from the finger contact sensors and compute the critical coefficient $\mu_{\mathrm{crit}}=mg/N$. We then freeze the gripper command, set the contact friction to $\alpha\mu_{\mathrm{crit}}$, and run a 5\,s fixed-hold slip test for several multipliers $\alpha$. In this experiment, $\mu_{\mathrm{crit}}=0.0902$, $N\approx6.962$\,N, $mg=0.6278$\,N, and the object mass is $0.064$\,kg.

This threshold sweep complements the force-balance measurement above. Below the critical coefficient, all methods slip as expected. At and above the theoretical threshold, \method maintains the grasp throughout the full 5\,s test, while MuJoCo Euler still drops the object almost immediately. MuJoCo FastImplicit delays the slip substantially but does not complete the hold even at $1.10\mu_{\mathrm{crit}}$. Together, the two measurements show that the evaluated grasp is not merely successful at the task level: \method also maintains a consistent force balance and preserves the hold under near-critical friction conditions.

\subsection{Normal Force Stability in Rolling Friction}
We tested a scenario \ref{fig:ball_falling_scene} where a small ball falls onto an inclined plane, with the rolling friction coefficient slightly larger than the theoretical threshold required for it to stop. In MuJoCo, during the first few frames of contact with the inclined plane, the ball experiences a large normal force that pushes it away from the surface, causing the normal force to drop to zero. The ball then falls back onto the plane, generating another large normal force. This process repeats continuously until the ball leaves the plane. In other words, the ball keeps bouncing down the inclined plane without stopping, with the normal force shaking between $0$ and $500$\,N. In contrast, in \method, the normal force experienced by the ball on the inclined plane eventually converges stably to the theoretical value, and the ball is able to come to a stop on the plane.

The sphere is a homogeneous ball with a mass of $10$\,kg, and the angle between the inclined plane and the ground is approximately $20^\circ$. Theoretically, as long as the rolling friction coefficient is greater than $0.1823$, the sphere should be able to decelerate to a stop on the inclined plane, so we set the rolling friction coefficient to $0.183$. The normal force acting on the sphere should be $92.165$\,N.
We can see from Fig.~\ref{fig:rolling_friction_comparison} that MuJoCo exhibits high-frequency shake while \method demonstrates stable convergence.

\section{3DGS Asset and Rendering}
\label{app:assets}

\subsection{Assets Generation}
\label{app:bridge_gs}
Building upon the widely used Bridge-v2 dataset\footnote{H. Walke et al., ``BridgeData V2: A Dataset for Robot Learning at Scale,'' in \textit{Conference on Robot Learning (CoRL)}, 2023.}, we introduce the Bridge-GS dataset, a large-scale collection of simulation-ready 3D visual assets produced by our automated reconstruction pipeline. Bridge-v2 spans 24 scene categories across five object families; our pipeline has produced thousands of usable Bridge-GS scenes, with successful reconstructions for most scenes after automatic processing and filtering. Dataset-scale generation is run as an offline, parallel pipeline across multiple GPUs rather than as serial per-scene processing. While the original Bridge-v2 dataset primarily consists of RGB images and robot trajectories, Bridge-GS significantly enriches this data by providing fully reconstructed scene-level and object-level 3D Gaussian Splatting (3DGS) representations, along with object-level meshes, 6D object poses, and calibrated camera intrinsics and extrinsics.

Figure \ref{fig:gs_datasets} illustrates samples from the Bridge-GS dataset. The dataset covers diverse real-world scenes reconstructed as photorealistic 3DGS environments for robot interaction. Each column represents a distinct scene processed by our pipeline. The top row displays the original RGB images from the Bridge-v2 dataset. The subsequent rows show the intermediate and final outputs of our pipeline: the estimated depth maps used for geometry estimation, the instance segmentation masks identifying interactable objects, and the final composited 3DGS assets rendered in the simulation environment. Challenging cases include heavy occlusion or stacking, transparent or highly reflective objects, and foundation-model errors that require filtering. This rich set of 3D annotations empowers researchers to train visuomotor policies in high-fidelity simulated replicas of real-world environments.

In addition to Bridge-v2, we further validate our pipeline using the InteriorGS dataset\footnote{SpatialVerse Research Team, Manycore Tech Inc., ``InteriorGS: A 3D Gaussian Splatting Dataset of Semantically Labeled Indoor Scenes,'' 2025. \url{https://huggingface.co/datasets/spatialverse/InteriorGS}}. Although InteriorGS provides ground-truth 3DGS representations, we utilize it strictly as a source of diverse indoor RGB imagery. We render 2D snapshots from the scenes and feed them into our pipeline as raw input, without accessing the underlying 3D data. As shown in the bottom half of Figure~\ref{fig:gs_datasets}, our pipeline successfully reconstructs these complex indoor environments into simulation-ready visual assets---recovering geometry, segmentation, and 3DGS representations purely from the rendered images. This demonstrates the pipeline's robustness and its capability to generalize to a wide variety of indoor settings beyond the specific domain of Bridge-v2.

\begin{figure*}[t]
    \centering
    \begin{subfigure}{\linewidth}
        \centering
        \includegraphics[width=0.75\linewidth]{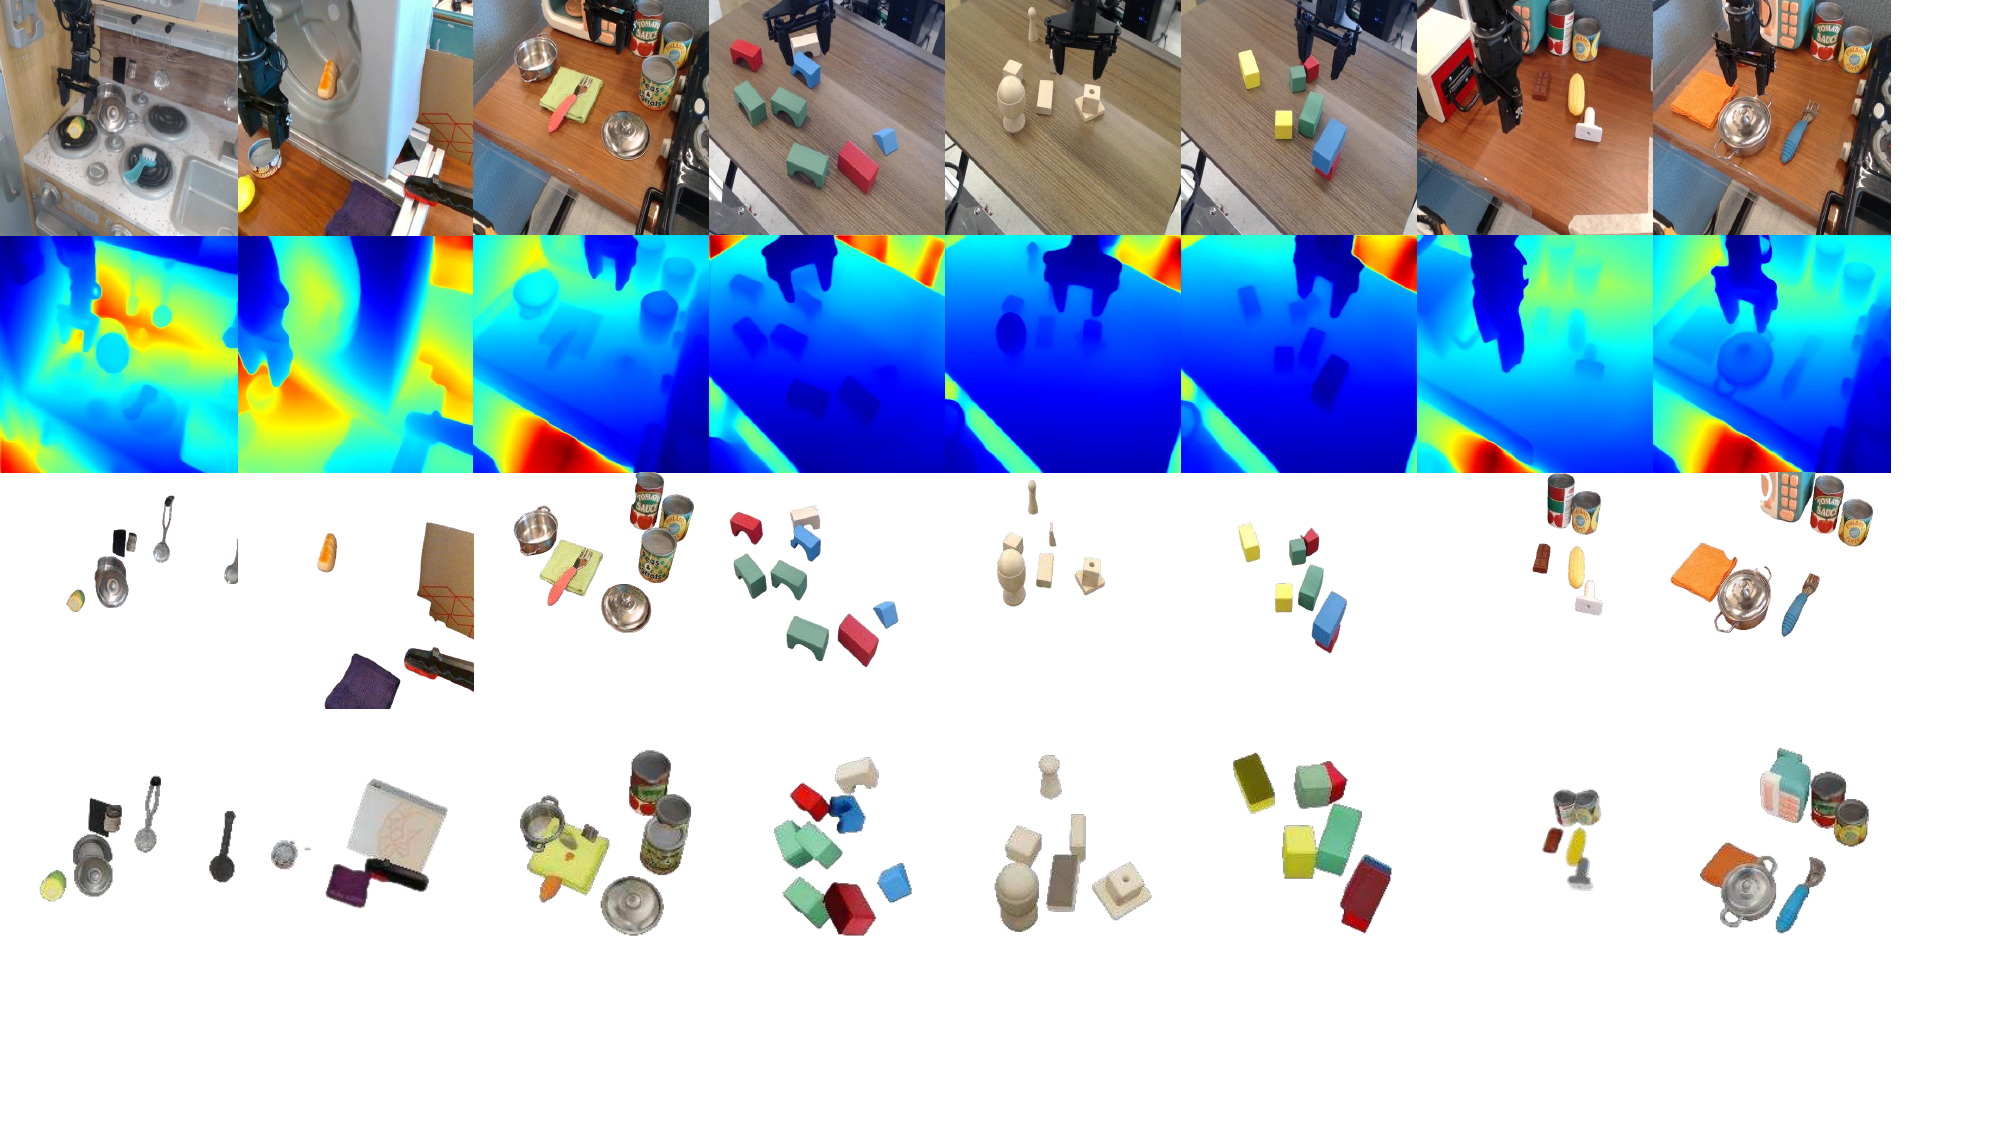}
        \label{fig:bridge_gs}
    \end{subfigure}
    \vspace{1em}
    \begin{subfigure}{\linewidth}
        \centering
        \includegraphics[width=0.75\linewidth]{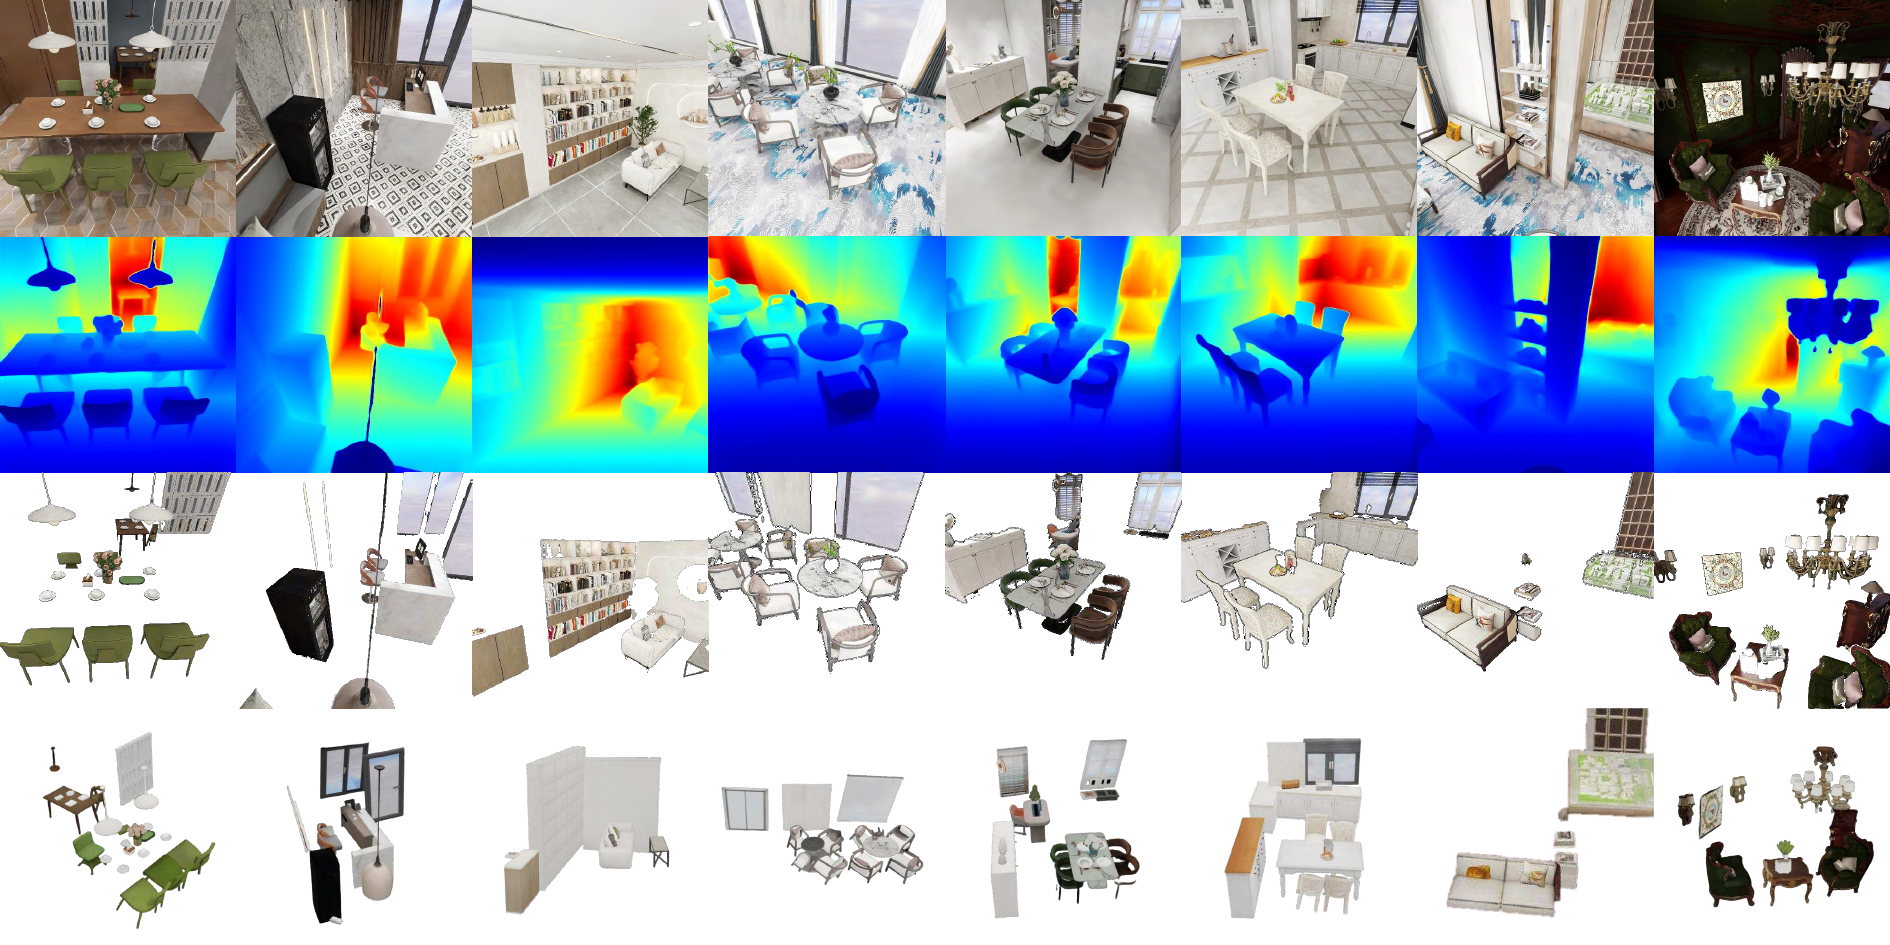}
        \label{fig:interior_gs}
    \end{subfigure}
    \caption{Visual results of the asset generation pipeline on (top) Bridge-GS and (bottom) InteriorGS datasets. The rows display: (1) Original RGB images; (2) Estimated depth maps; (3) Instance segmentation masks; and (4) Reconstructed simulation-ready 3DGS assets.}
    \label{fig:gs_datasets}
\end{figure*}

\subsection{RLGK}
\label{appendix:rlgk}
Rigid-Link Gaussian Kinematics (RLGK) is a mechanism designed to efficiently synchronize the state of millions of 3D Gaussians with the low-dimensional rigid body states derived from the physics engine. The core logic of RLGK is to map the update of high-dimensional visual representations to low-dimensional rigid body transformations, executing the synchronization process via massively parallelized vector operations on the GPU. Importantly, our implementation is optimized for \textbf{batched environments}, enabling the simultaneous simulation and rendering of $B$ parallel scenes (e.g., $B=2048$) using a single geometry template.

During the initialization phase, we upload a single "template" of the scene's Gaussians to GPU memory. We assign a rigid body index $k \in \{0, \dots, N_{bodies}\}$ to each Gaussian $g_i$ and store the initial local configuration $\{ p_{local}^i, q_{local}^i \}$ relative to the body frame.
At runtime, the physics engine outputs a batch of global poses $\mathbf{S}_t \in \mathbb{R}^{B \times N_{bodies} \times 7}$ containing the state of every rigid body in every parallel environment. RLGK performs a batched gather operation to retrieve the transform for every Gaussian across all environments simultaneously. The new global state for the $j$-th environment and $i$-th Gaussian is computed via:
\begin{align}
p_{world}^{(j,i)} &= R(q_k^{(j,t)}) p_{local}^i + t_k^{(j,t)} \\
q_{world}^{(j,i)} &= q_k^{(j,t)} \otimes q_{local}^i
\end{align}

This design allows for updating $B \times M$ points (where $M \approx 10^6$) in sub-milliseconds. By broadcasting the single template geometry $\{p_{local}^i\}$ across $B$ environments, we minimize memory bandwidth usage. The algorithmic description is provided in Algorithm \ref{alg:rlgk}.

\begin{algorithm}[h]
\centering
\caption{Batched Rigid-Link Gaussian Kinematics (RLGK)}
\label{alg:rlgk}
\begin{algorithmic}[1]
\State \textbf{Input:} Template Gaussians $\mathcal{G} = \{g_1, \dots, g_M\}$, Batch Size $B$
\State \textbf{Pre-computation:}
\For{each Gaussian $g_i \in \mathcal{G}$}
    \State Identify body index $k_i \in \{1, \dots, N_{bodies}\}$
    \State Store local pose: $p_{local}^i, q_{local}^i$
    \State $IndexMap[i] \gets k_i$
\EndFor
\State \textbf{Runtime Loop (at step $t$):}
\State Receive batch body states $\mathbf{S}_t \in \mathbb{R}^{B \times N_{bodies} \times 7}$
\State Transfer $\mathbf{S}_t$ to GPU memory
\State \textit{// Massive Parallel Update for $(B \times M)$ Gaussians}
\State $K \gets \mathbf{S}_t[:, IndexMap]$ \Comment{Gather: $(B, N_{bodies}) \to (B, M)$}
\State $\mathbf{P}_{world} \gets \text{Transform}(\mathbf{P}_{local}, K.p, K.q)$ \Comment{Broadcast $(1, M)$ to $(B, M)$}
\State $\mathbf{Q}_{world} \gets K.q \otimes \mathbf{Q}_{local}$
\State Update renderer buffers with batched state $\mathbf{P}_{world}, \mathbf{Q}_{world}$
\end{algorithmic}
\end{algorithm}

\subsection{Consistency of Policy Performance between Simulation and Real World}

\begin{figure}[h!]
    \centering
    \includegraphics[width=0.75\linewidth]{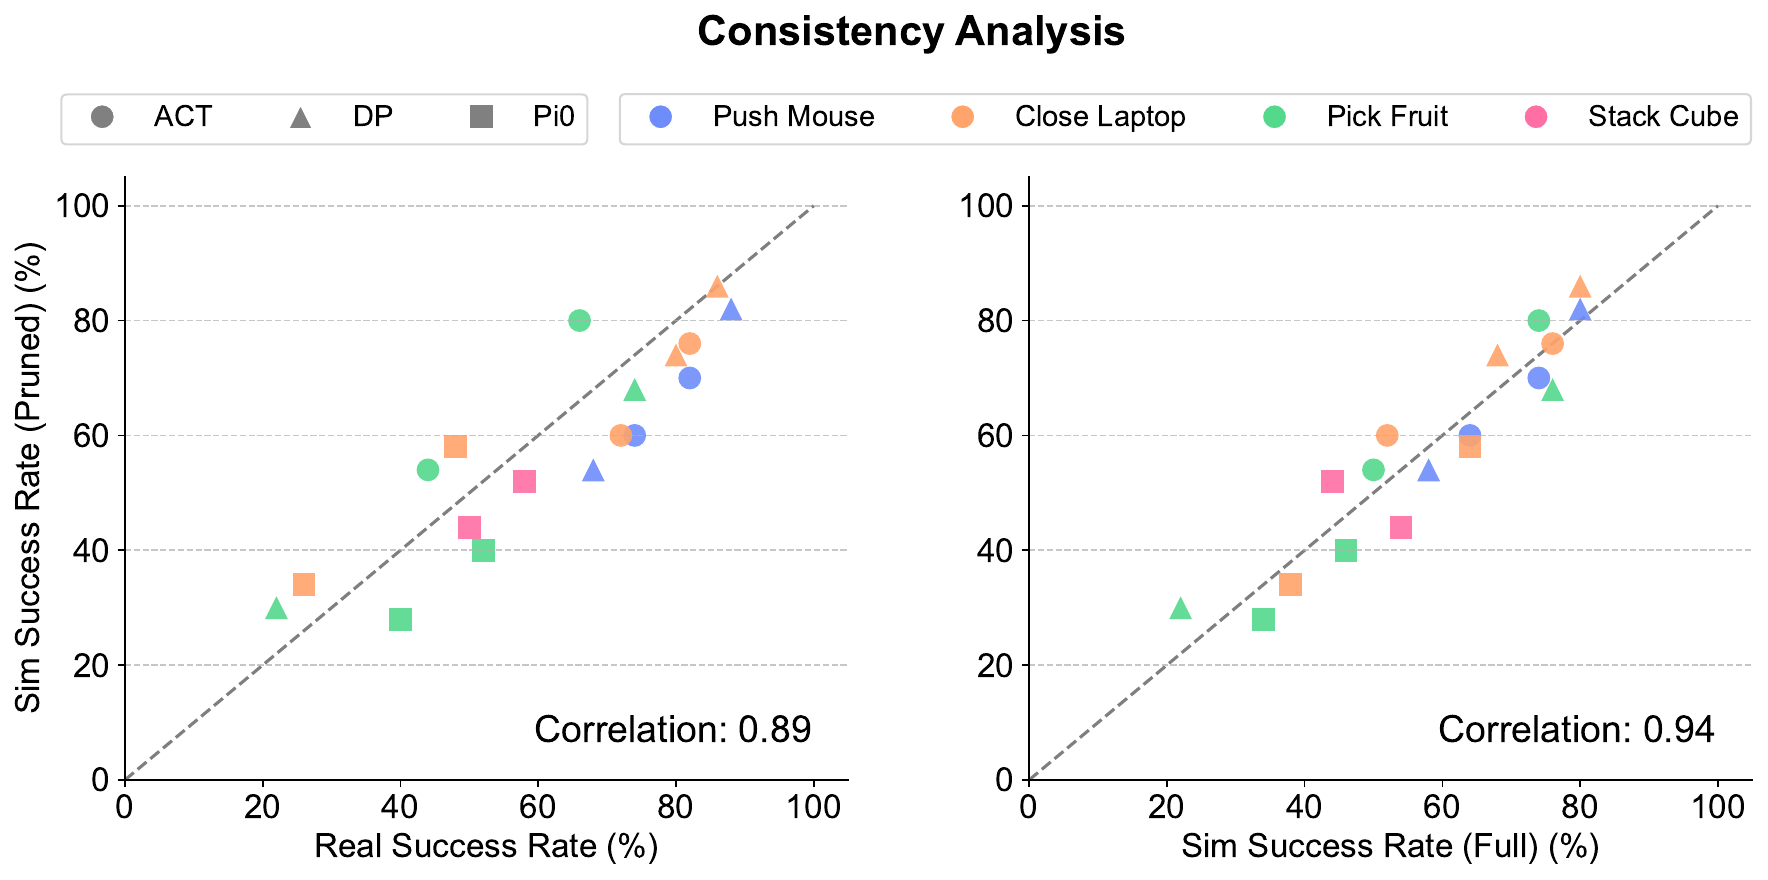}
    \caption{We compare the success rates of different policies in simulation and the real world on various tasks.}
    \label{fig:consistency_analysis}
\end{figure}

We present the consistency analysis in Figure \ref{fig:consistency_analysis}. We evaluated three representative imitation learning algorithms—ACT, Diffusion Policy (DP), and $\pi_0$—across four diverse manipulation tasks: Push Mouse, Close Laptop, Pick Fruit, and Stack Cube.
First, our experiments demonstrate a strong correlation ($0.89$) between simulation and real-world success rates, indicating good sim-real agreement across different policy architectures and task scenarios. Second, as detailed in Section \ref{sec:renderer}, our efficient pruning strategy significantly reduces the number of Gaussians while maintaining high visual fidelity. The comparison between full and pruned 3DGS rendering shows that this reduction in point count has a negligible impact on the validation success rate of imitation learning policies. This confirms that our compression strategy effectively preserves the essential visual features required for policy learning while significantly lowering the method's computational footprint.

\section{Locomotion}
\label{app:locomotion}

\subsection{Environment Setup}
In this task, we consider two environments: a Unitree Go2 quadruped environment and a Unitree G1 humanoid environment.

\subsection{Training Details}

\noindent\textbf{Observation and Action.}
We use a unified observation space for all environments:
\begin{itemize}
    \item Gravity projected in body frame
    \item Angular velocity
    \item Joint positions
    \item Joint velocities
    \item Previous action
    \item Velocity commands
    \item Phase
\end{itemize}
The action space is defined as absolute joint position with a default offset:
\begin{equation}
q_{t}=q_{d}+k_{a}a
\end{equation}
where $k_a$ is the action scale, $q_d$ is the default position and $a$ is the action. We employ a PD controller to map joint position to torque:
\begin{equation}
\tau =k_p(q_t-q)-k_d\dot{q}
\end{equation}

\smallskip
\noindent\textbf{Domain Randomization.}
For better sim-to-real transfer, we employ domain randomization by randomizing the following components:
\begin{itemize}
    \item \textbf{Sensor noise}: We add Gaussian noise to the data from each sensor.
    \item \textbf{Physical parameters}: Noise is introduced to physical quantities that are difficult to measure accurately, such as inertia and the center of mass, to enhance the robustness of the policy.
\end{itemize}

\smallskip
\noindent\textbf{Reward Function.}
The training rewards are detailed in Table \ref{tb:reward_design}.

\begin{table}[h]
    \centering
    \caption{Reward Functions for Locomotion Tasks} 
    \label{tb:reward_design}
    \begin{tabular}{lccc}
        \toprule
        \textbf{Reward} & \textbf{Go2 Weight} & \textbf{G1 Weight} & \textbf{Expression} \\
        \midrule
        Joint torques & -1e-5 & -1e-5& $|\tau|^2$ \\
        Dof pos limits & -1 & & $|q|-q_{max}$ \\
        Feet air time & 1 & 2 & $(t_{air}-t_{threshold})*(1-Q_{d})$ \\
        Speed tracking   & 1 & 1& $e^{-[\frac{(v_{com}-v_d)^2}{0.01}+\frac{(\omega_{com}-\omega_d)^2}{0.005}]}$ \\
        Z-axis velocity & -2 & -4 & $|v_{CoM,z}|^2$ \\
        Action rate & -0.02 & -0.01 & $|\triangle q_{last}-\triangle q|^2$ \\
        Joint acc & -2.5e-7 & -2.5e-7 & $|\frac{\dot{q}_{last}-\dot{q}}{\triangle t}|^2$ \\
        \bottomrule
    \end{tabular}
\end{table}

\smallskip
\noindent\textbf{Network Architecture.}
We employ an asymmetric actor–critic setup, in which the policy network (actor) and the value network (critic) receive different observation inputs. The policy network is fed with the aforementioned observations, while the value network additionally receives uncorrupted versions of these signals and extra sensor readings such as contact forces, perturbation forces, and linear velocity. Both policy and value networks use a three-layer multilayer perceptron (MLP) with hidden sizes of 256, 128, and 64.

\smallskip
\noindent\textbf{Training Curve.}
Learning curves for the G1 and Go2 Joystick tasks are shown in Figure~\ref{fig:g1_reward} and Figure~\ref{fig:go2_reward}, respectively.

\begin{figure}[h]
    \centering
    \includegraphics[width=0.5\linewidth]{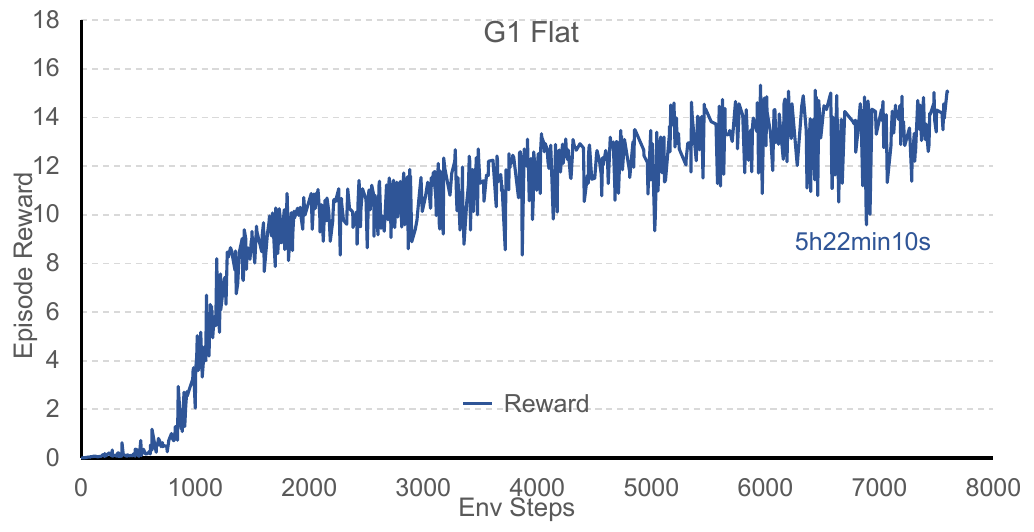}
    \caption{Learning curves for the G1 Joystick task.}
    \label{fig:g1_reward}
\end{figure}

\begin{figure}[h]
    \centering
    \includegraphics[width=0.5\linewidth]{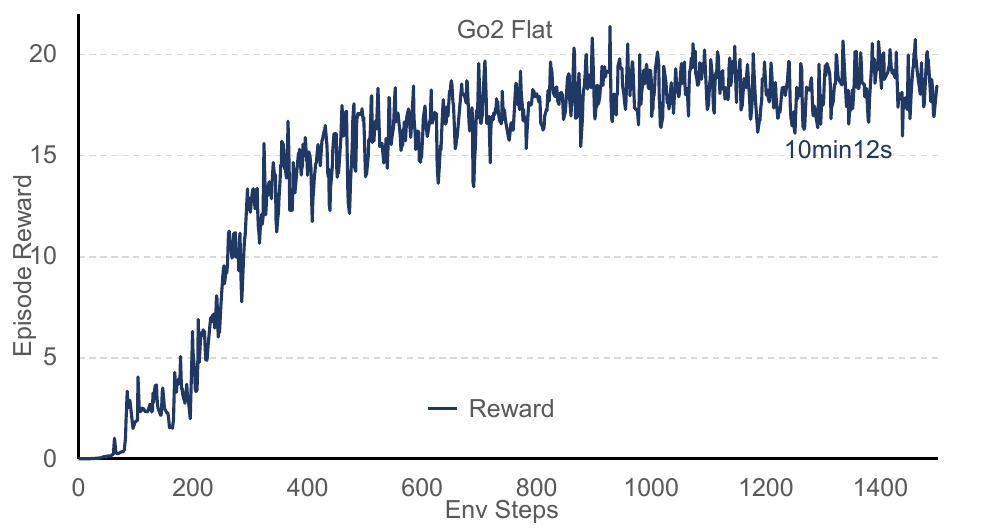}
    \caption{Learning curves for the Go2 Joystick task.}
    \label{fig:go2_reward}
\end{figure}

\subsection{Specialized Perception}
To enable robust locomotion across diverse terrains, we provide a suite of high-fidelity exteroceptive sensors compatible with various robot embodiments. As illustrated in Figure \ref{fig:loco_lidar}, these sensors can be flexibly configured to suit different tasks and morphologies.

\smallskip
\noindent\textbf{Height Scan.}
The Height Scan sensor projects a grid of ray-casts downwards around the robot base to sample terrain elevation relative to the body frame. This local height map provides high-frequency terrain geometry information, essential for traversability analysis on rough terrain. In our benchmarks, we equip the Unitree Go2 quadruped with this sensor to facilitate adaptive gait generation on uneven surfaces.

\smallskip
\noindent\textbf{LiDAR.}
The 3D LiDAR sensor performs omnidirectional or bounded ray-casting to generate a sparse point cloud of the environment. This modality is critical for obstacle detection, mapping, and navigation in cluttered spaces. We demonstrate its integration on the Unitree G1 humanoid for humanoid locomotion tasks.

Both sensors leverage our batched ray-casting engine to maintain high throughput during massive parallel training.

\begin{figure}[h]
    \centering
    \includegraphics[width=0.75\linewidth]{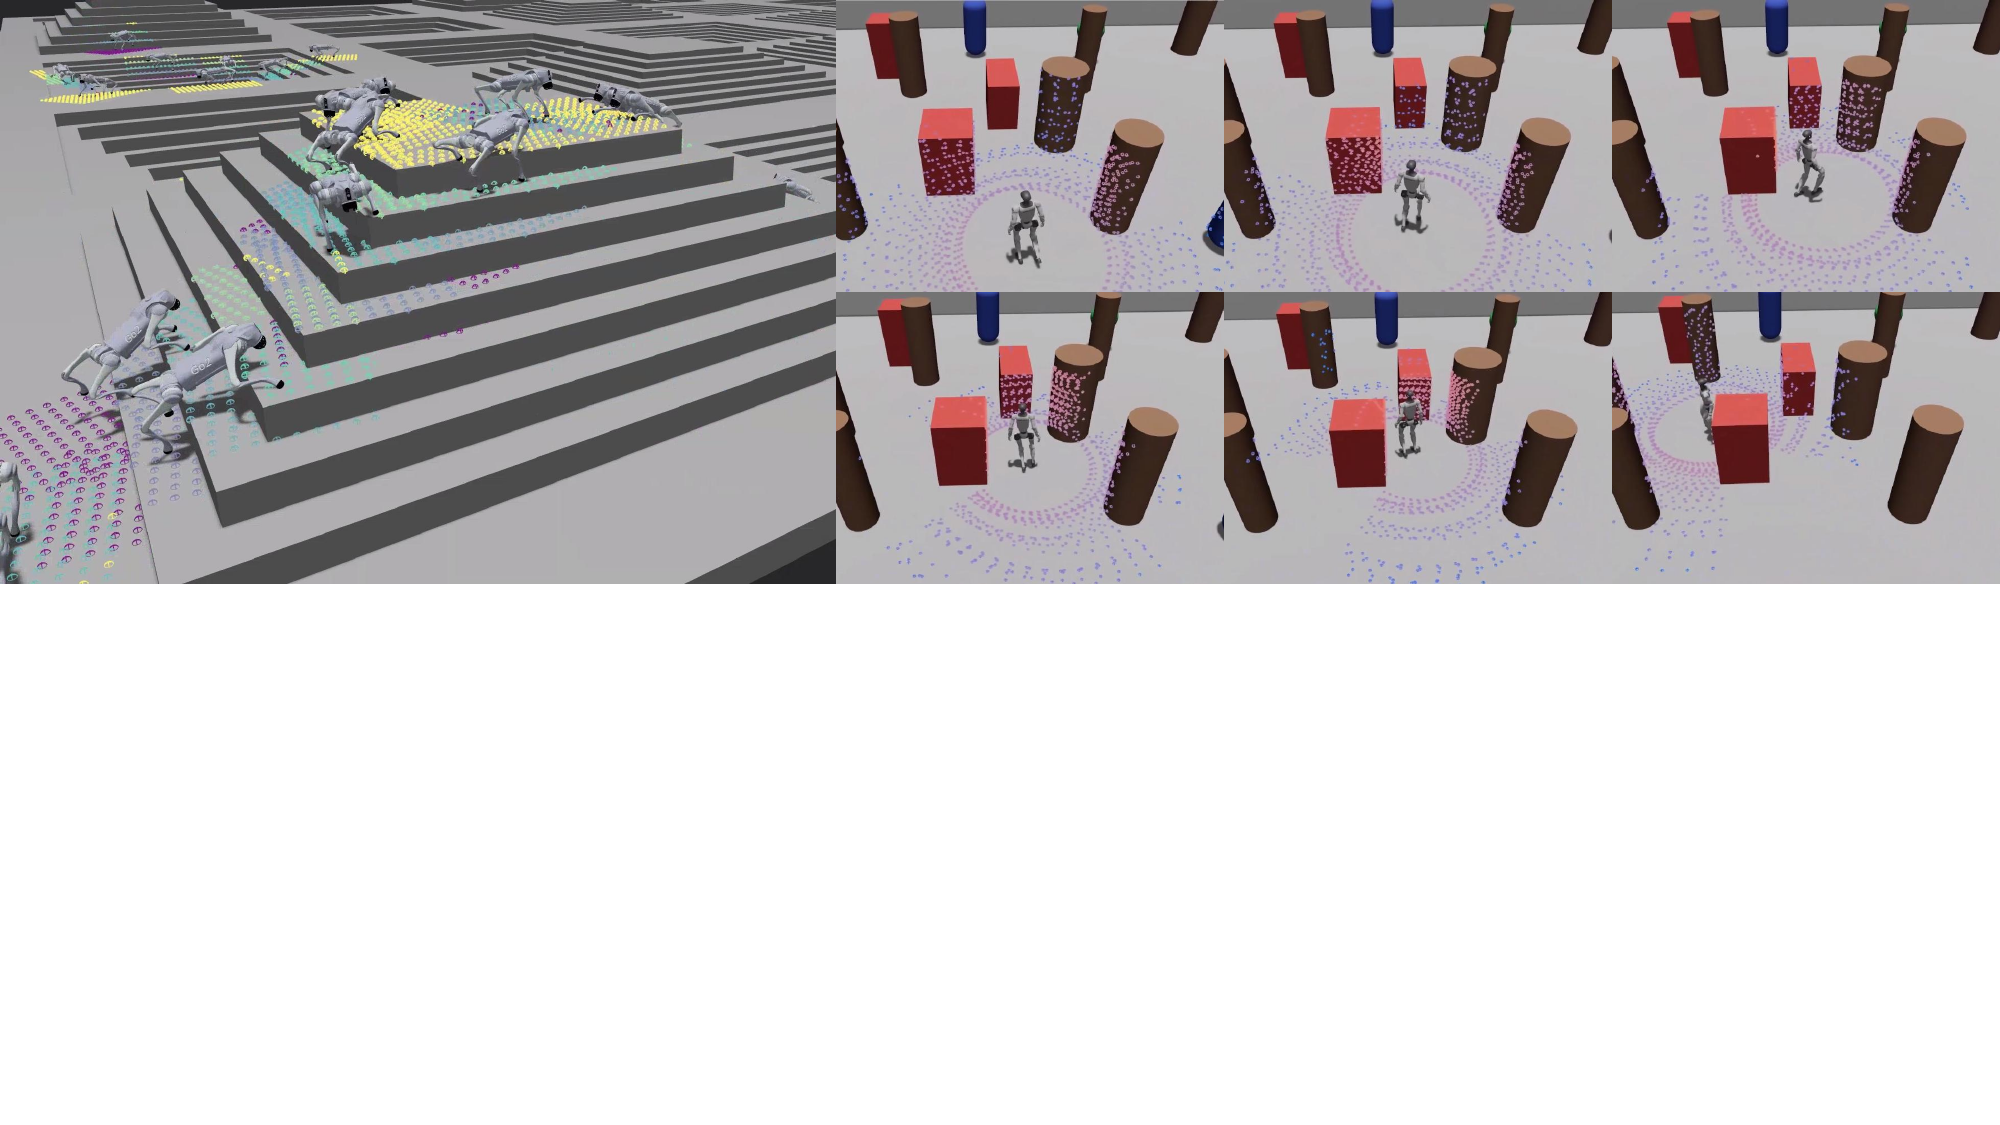}
    \caption{Perception setups for locomotion tasks. \textbf{Left:} The Unitree Go2 robot utilizing a Height Scan sensor to perceive terrain geometry on rough terrain. \textbf{Right:} The Unitree G1 humanoid equipped with a LiDAR sensor for environmental awareness.}
    \label{fig:loco_lidar}
\end{figure}

\section{Manipulation}
\label{app:manipulation}

\subsection{Environment Setup}
The environment used is AIRBOT Play PickCube, as shown in Figure \ref{fig:pick_cube}. The objective of this task is to control the robotic arm to grasp a cube placed on the table and lift it to a specified target position.

\begin{figure}[h]
    \centering
    \includegraphics[width=0.5\linewidth]{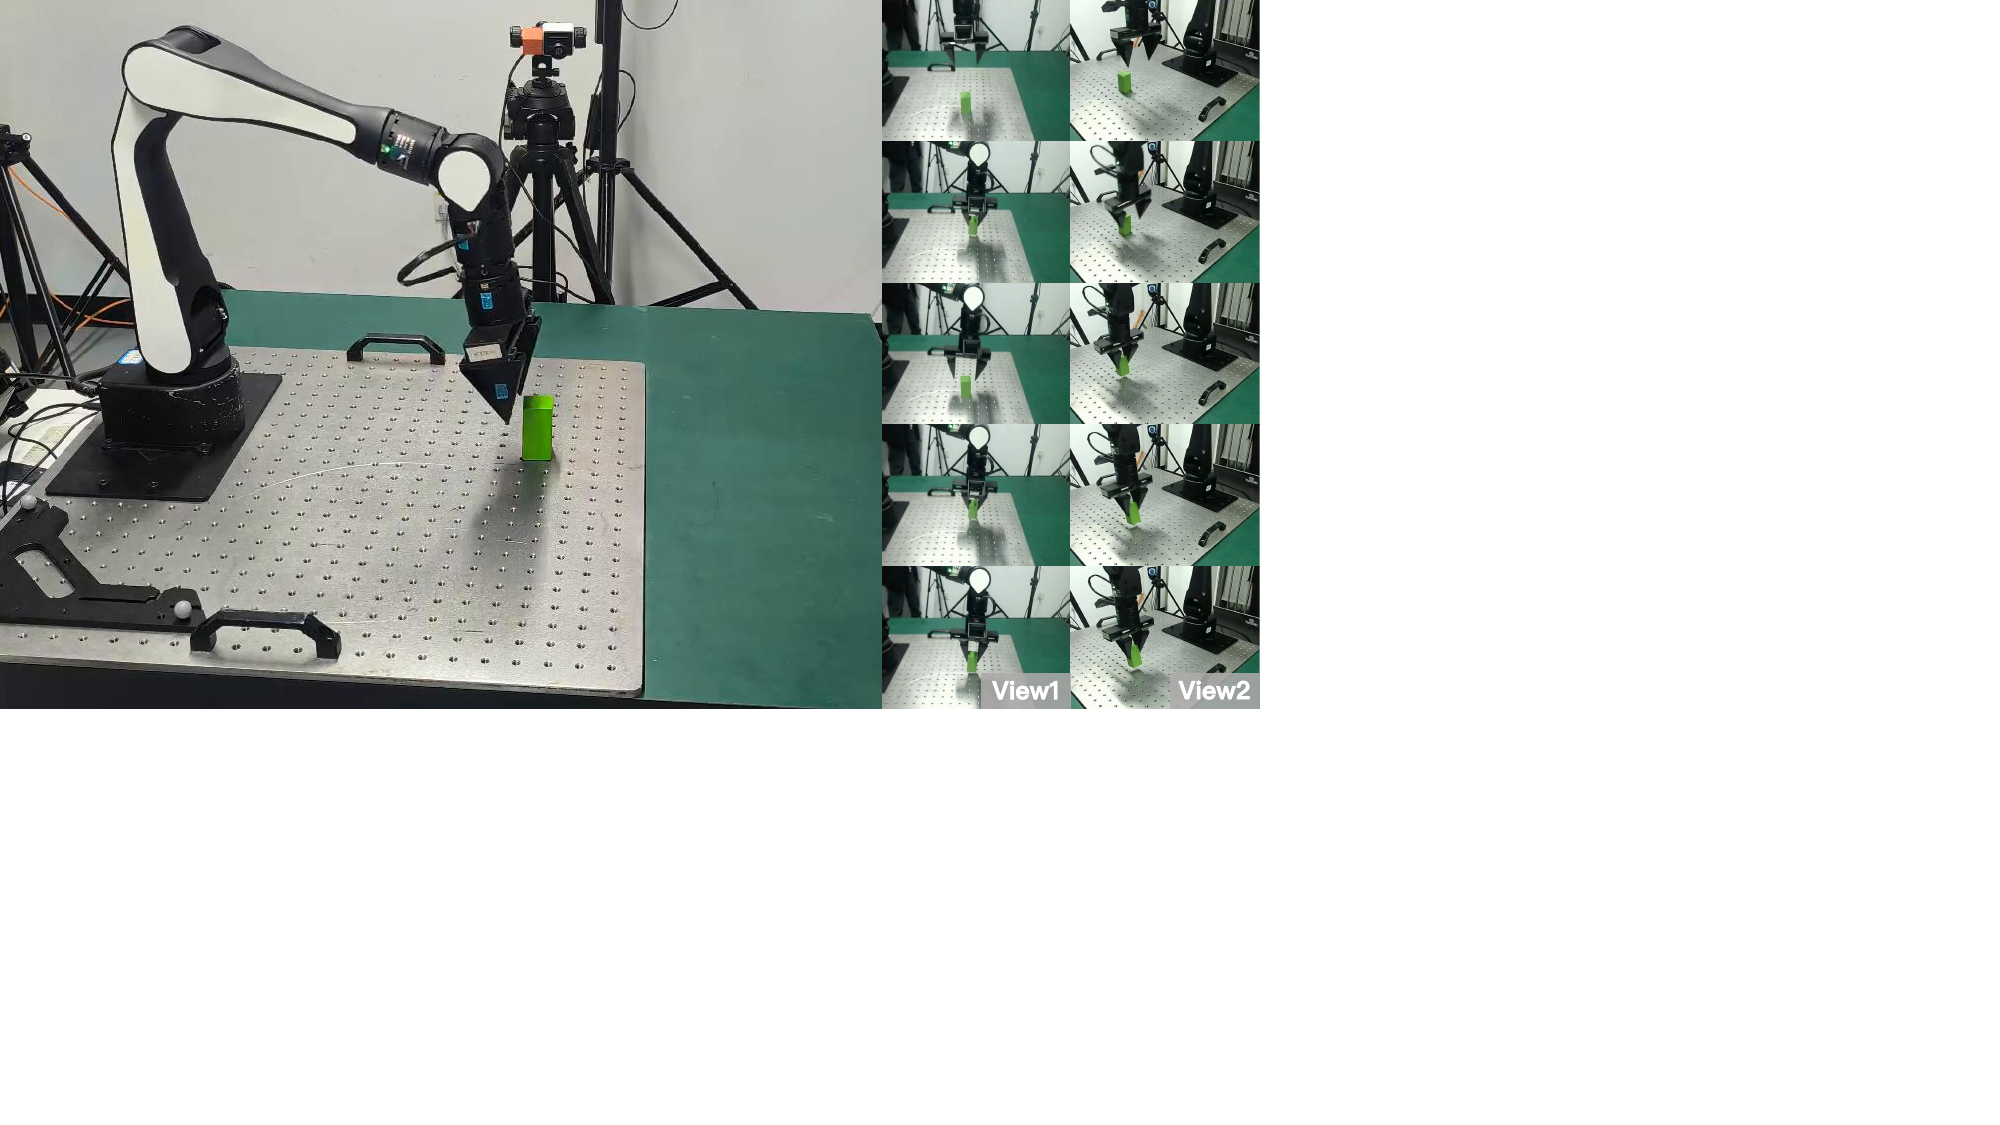}
    \caption{The AIRBOT Play PickCube manipulation environment setup. The robot needs to grasp the green cube and lift it to the target position.}
    \label{fig:pick_cube}
\end{figure}

\subsection{Training Details}

\noindent\textbf{Observation and Action.}
\begin{itemize}
    \item \textbf{Observation Space}
    \begin{itemize}
        \item Arm joint positions
        \item Gripper position
        \item Target position
        \item Joint tracking error: the difference between the current control command and the robot's current joint positions
        \item Two input RGB images
    \end{itemize}
    \item \textbf{Action Space}
    \begin{itemize}
        \item 6 DoF joint positions
        \item 1 Gripper position
    \end{itemize}
\end{itemize}

\smallskip
\noindent\textbf{Goal-Conditioned RL Setup.}
The observed \emph{target position} is the static placement goal (fixed within each episode); the block's initial 3D pose is randomized per reset (see below) and is \emph{not} observed, so grasping must rely on the two RGB streams---removing them drops zero-shot success to 0\%.

\smallskip
\noindent\textbf{Domain Randomization.}
\begin{itemize}
    \item \textbf{Camera poses}: We perform multi-camera domain randomization by perturbing each camera's extrinsics independently for every parallel world. For each camera, we add a per-axis uniform translation offset in the range $\pm0.02$ m to the nominal camera position, and apply a small random rotation by sampling a random 3D axis and a rotation angle uniformly up to $5^\circ$ (axis--angle $\to$ quaternion, then composed with the original orientation).
    \item \textbf{Box initial and target positions}: At each reset, we randomize the initial 3D positions of both the box and the target by sampling a small uniform offset around their nominal location. The box is perturbed within $\pm5$ cm in x, $\pm10$ cm in y, and 0 cm in z, while the target is perturbed within 0 cm in x, $\pm10$ cm in y, and 3--8 cm upward in z (all relative to the same nominal reference).
    \item \textbf{Image-level appearance}: We additionally apply per-environment color augmentation to rendered RGB observations, randomizing brightness, contrast, and exposure to mitigate residual photometric mismatch with the real camera (3DGS bakes static lighting; cf. Sec.~\ref{sec:limitations}).
\end{itemize}

\smallskip
\noindent\textbf{Reward Function.}

\begin{table}[h]
    \centering
    \caption{Reward Functions for PickCube Manipulation}
    \label{tab:pick_rewards}
    \begin{tabular}{@{}l c l@{}}
        \toprule
        \textbf{Reward} & \textbf{Weight} & \textbf{Expression} \\
        \midrule
        Gripper--Box Proximity & 5.0 & $1 - \tanh\!\big(5\,\lVert \mathbf{p}_{\mathrm{box}} - \mathbf{p}_{\mathrm{grip}} \rVert\big)$ \\
        Box--Target Tracking & 5.0 & $\Big(1 - \tanh\!\big(5\,\lVert \mathbf{p}_{\mathrm{tgt}} - \mathbf{p}_{\mathrm{box}} \rVert\big)\Big)\,\mathbb{I}_{\mathrm{reach}}$ \\
        No Floor Collision & 0.25 & $1 - \mathbb{I}_{\mathrm{floor}}$ \\
        No Box Collision & 0.5 & $1 - \mathbb{I}_{\mathrm{hand\text{-}box}}$ \\
        Gripper Closing & 20.0 & $\Big(1 - \frac{\lvert u_g - u_{\min} \rvert}{u_{\max}-u_{\min}}\Big)\,\mathbb{I}_{\mathrm{reach}}$ \\
        Lifted (sparse) & 8.0 & $\mathbb{I}\big(p^{z}_{\mathrm{box}} > p^{z}_{\mathrm{box,0}} + 0.005\big)\,\mathbb{I}_{\mathrm{reach}}$ \\
        Success (sparse) & 10.0 & $\mathbb{I}\big(\lVert \mathbf{p}_{\mathrm{box}} - \mathbf{p}_{\mathrm{tgt}} \rVert < \epsilon\big)$ \\
        \bottomrule
    \end{tabular}
\end{table}

\smallskip
\noindent\textbf{Notation.}
$\mathbf{p}_{\mathrm{box}}$ is the box position, $\mathbf{p}_{\mathrm{tgt}}$ is the target (mocap) position, and $\mathbf{p}_{\mathrm{grip}}$ is the gripper site position.
$p^{z}_{\mathrm{box}}$ and $p^{z}_{\mathrm{box,0}}$ denote the current and initial box height, respectively.
$u_g$ is the gripper control command (last control dimension), with limits $u_{\min}$ and $u_{\max}$.
$\mathbb{I}(\cdot)$ is the indicator function.
$\mathbb{I}_{\mathrm{reach}} = \mathbb{I}(\lVert \mathbf{p}_{\mathrm{box}} - \mathbf{p}_{\mathrm{grip}} \rVert < 0.015)$ gates rewards that should only activate after the gripper reaches the box.
$\mathbb{I}_{\mathrm{floor}}$ and $\mathbb{I}_{\mathrm{hand\text{-}box}}$ indicate floor contact and hand--box collision as detected by contact sensors.
$\epsilon$ is the success threshold (set to $0.01$ in our experiments).
The sparse bonuses "Lifted" and "Success" are applied in the vision setting.
The episode reward is computed as $\mathrm{clip}(\sum_i w_i r_i, -10^4, 10^4)$.

\smallskip
\noindent\textbf{Termination.} The episode terminates when any of the following conditions becomes true: (i) the box goes out of bounds (any coordinate exceeds 1.0 m in magnitude, or the box drops below its initial height by more than 0.01 m), (ii) the simulation state becomes non-finite (any NaN in qpos or qvel), or (iii) the task is successful.

\smallskip
\noindent\textbf{Network Architecture and Hyperparameters.}
We used the same vision PPO network as in Mujoco Playground, except that we modified the output features of the CNN encoders for both the actor and critic to 16. The training hyperparameters are shown in Table \ref{tab:ppo_hyperparameters}.

\begin{table}[h]
    \centering
    \caption{PPO Hyperparameters for Manipulation}
    \label{tab:ppo_hyperparameters}
    \begin{tabular}{lc}
        \toprule
        \textbf{Hyperparameter} & \textbf{Default Value} \\
        \midrule
        empirical\_normalization & True \\
        num\_minibatches & 8 \\
        discounting & 0.97 \\
        learning\_rate & $1\mathrm{e}{-3}$ \\
        num\_envs & 2048 \\
        num\_steps\_per\_env & 40 \\
        value\_loss\_coef & 1.0 \\
        use\_clipped\_value\_loss & True \\
        clip\_param & 0.2 \\
        entropy\_coef & 0.01 \\
        num\_learning\_epochs & 4 \\
        schedule & adaptive \\
        gamma & 0.97 \\
        lam & 0.95 \\
        desired\_kl & 0.01 \\
        max\_grad\_norm & 1.0 \\
        \bottomrule
    \end{tabular}
\end{table}

\smallskip
\noindent\textbf{Training Curve.}
In Figure~\ref{fig:pickcube_reward} we report environment steps versus reward across 4 seeds on a single A100 GPU.

\begin{figure}[h]
    \centering
    \includegraphics[width=0.5\linewidth]{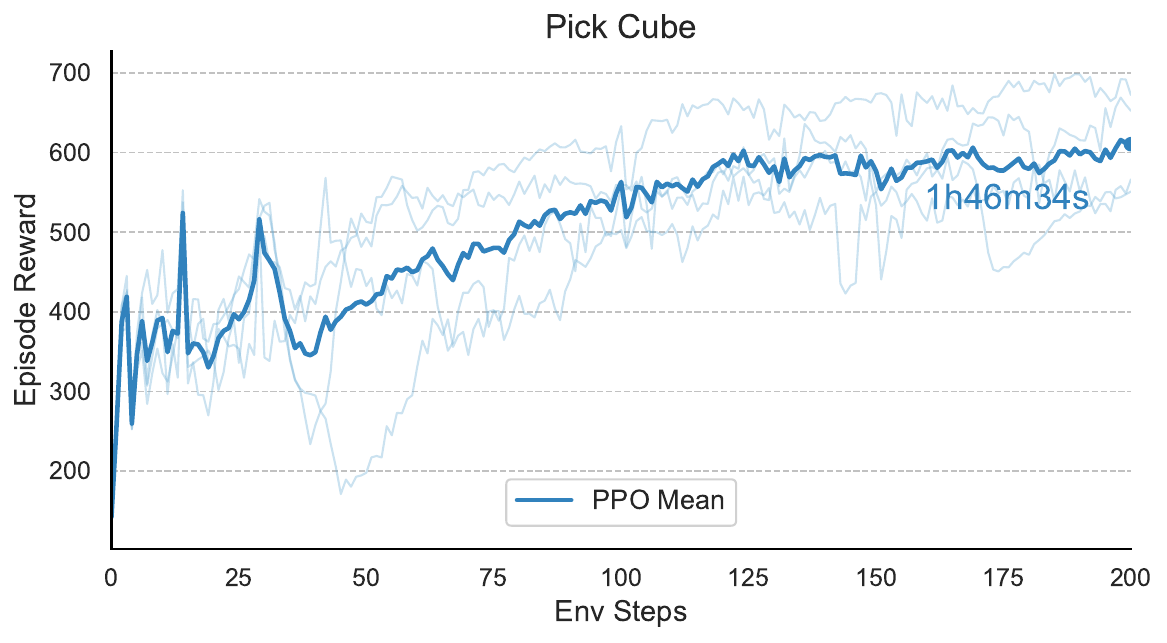}
    \caption{Learning curves for the PickCube manipulation task.}
    \label{fig:pickcube_reward}
\end{figure}

\section{Navigation}
\label{app:navigation}

\subsection{Task Definition}
We evaluate a simplified visual goal-seeking task in \textbf{structured indoor scenes}. The Unitree Go2 robot is required to locate and approach a \textbf{red} traffic cone based on egocentric RGB observations, within a time limit of $T_{\max} = 25$ seconds. The task is successful when the Euclidean distance between the robot's base and the center of the target cone falls below a threshold $\epsilon = 0.35$ meters. The robot's initial pose and the cone position are randomized at episode start (see Domain Randomization).

\subsection{Scene Reconstruction and Rendering}
The simulation scene is captured with an RGB camera and reconstructed using the PGSR algorithm to obtain a 3D representation suitable for rendering. During training, RGB observations are rendered from the robot dog's egocentric viewpoint (camera pose and intrinsics aligned with the Go2's onboard camera) so that the policy receives first-person visual input consistent with real-world deployment.

\subsection{Training Details}
\noindent\textbf{Observation and Action Space.}
We use a hierarchical setup: a high-level navigation policy runs at 5\,Hz and outputs velocity commands; a low-level locomotion controller runs at 50\,Hz and maps commands plus proprioception to joint targets. The low-level controller is first pre-trained with PPO under domain randomization and remains frozen during navigation training.

The observation space for the high-level policy is 228-dimensional: (1)~\textbf{Visual features} (192 dimensions), i.e., image embeddings from a Vision Transformer (ViT) encoder; (2)~\textbf{Task command} (3 dimensions), a one-hot vector indicating the target color---in this simplified task only the red cone is used; (3)~\textbf{Proprioception} (33 dimensions), including base angular velocity, projected gravity, joint positions, joint velocities, and the previous action. The action space consists of 3 continuous velocity commands $\mathbf{v}_{\mathrm{cmd}} = (v_x, v_y, \omega_{\mathrm{yaw}})$, squashed by a Tanh activation and scaled to the robot's physical limits.

\noindent\textbf{Policy Architecture.}
The high-level policy uses an asymmetric Actor-Critic structure. The Actor takes the observations above and incorporates a \textbf{pre-trained ViT encoder} (frozen during navigation training) to extract features from $224 \times 224$ RGB images, followed by an LSTM to aggregate temporal information. The Critic uses the same visual and proprioceptive inputs and follows the asymmetric design described in the locomotion appendix. Both policy and value networks are optimized with PPO.

\smallskip
\noindent\textbf{Reward Function.}
The reward function is given in Table~\ref{tab:nav_rewards}. It combines a sparse success bonus for reaching the goal with dense terms for horizontal and vertical goal distance reduction, heading alignment, stopping near the goal, velocity tracking, and an action L2 penalty. 
We use the following notation for the reward terms. Let $\mathbb{I}(\cdot)$ denote the indicator function, $\mathbf{p}_{\mathrm{root},t}$ and $\mathbf{q}_{\mathrm{root},t}$ denote the robot root position and quaternion, and $R(\cdot)$ denote the corresponding rotation matrix. The head point is defined as $\mathbf{p}_{\mathrm{head},t}=\mathbf{p}_{\mathrm{root},t}+R(\mathbf{q}_{\mathrm{root},t})[0.332,0,0]^\top$, and $\mathbf{p}_{\mathrm{goal}}$ denotes the selected cone target after applying a $0.32$\,m vertical offset. We further define $d_t=\|\mathbf{p}_{\mathrm{head},t}-\mathbf{p}_{\mathrm{goal}}\|_2$, $e^z_t=|z_{\mathrm{root},t}-z_{\mathrm{goal}}|$, where $z_{\mathrm{root},t}$ and $z_{\mathrm{goal}}$ are the $z$ coordinates of $\mathbf{p}_{\mathrm{root},t}$ and $\mathbf{p}_{\mathrm{goal}}$, respectively. Finally, $\Delta\psi_t$ is the absolute wrapped yaw error between the robot heading and the goal direction, $\mathbf{v}_{\mathrm{cmd},t}=(v_x,v_y,\omega_z)$ is the velocity command, $\mathbf{v}^{xy}_{\mathrm{cmd},t}$ and $\omega^z_{\mathrm{cmd},t}$ are its planar and yaw components, $\mathbf{v}^{xy}_{\mathrm{base},t}$ and $\omega^z_{\mathrm{base},t}$ are root velocities in the base frame, and $\mathbf{a}_t$ is the high-level policy action.

\begin{table}[h]
\caption{Reward Function for High-Level Navigation Policy}
\label{tab:nav_rewards}
\centering
\begin{tabular}{llc}
\toprule
\textbf{Reward Term} & \textbf{Expression / Description} & \textbf{Weight} \\
\midrule
\multicolumn{3}{c}{\textit{Task Rewards}} \\
\midrule
Reach Goal & $\mathbb{I}(d_t < 0.35)$ & $0.5$ \\
Goal Distance & $(d_{t-1} - d_t) \cdot \mathbb{I}(d_t > 0.25)$ & $5.0$ \\
Goal Height Distance & $e^z_{t-1} - e^z_t$ & $30.0$ \\
Goal Heading & $1 - \frac{2\Delta\psi_t}{\pi} \cdot \mathbb{I}(d_t > 0.25)$ & $0.3$ \\
Stand Still at Goal & $\mathbb{I}(d_t < 0.25)/(\|\mathbf{v}_{\mathrm{cmd},t}\|_2 + 0.4)$ & $1.0$ \\
\midrule
\multicolumn{3}{c}{\textit{Tracking and Regularization}} \\
\midrule
Linear Velocity Tracking & $\exp(-\|\mathbf{v}^{xy}_{\mathrm{cmd},t} - \mathbf{v}^{xy}_{\mathrm{base},t}\|_2^2/0.5^2)$ & $0.2$ \\
Angular Velocity Tracking & $\exp(-|\omega^{z}_{\mathrm{cmd},t} - \omega^{z}_{\mathrm{base},t}|^2/0.5^2)$ & $0.2$ \\
Action L2 & $\|\mathbf{a}_t\|_2^2$ & $-0.002$ \\
\bottomrule
\end{tabular}
\end{table}

\begin{figure}[h]
    \centering
    \includegraphics[width=0.5\linewidth]{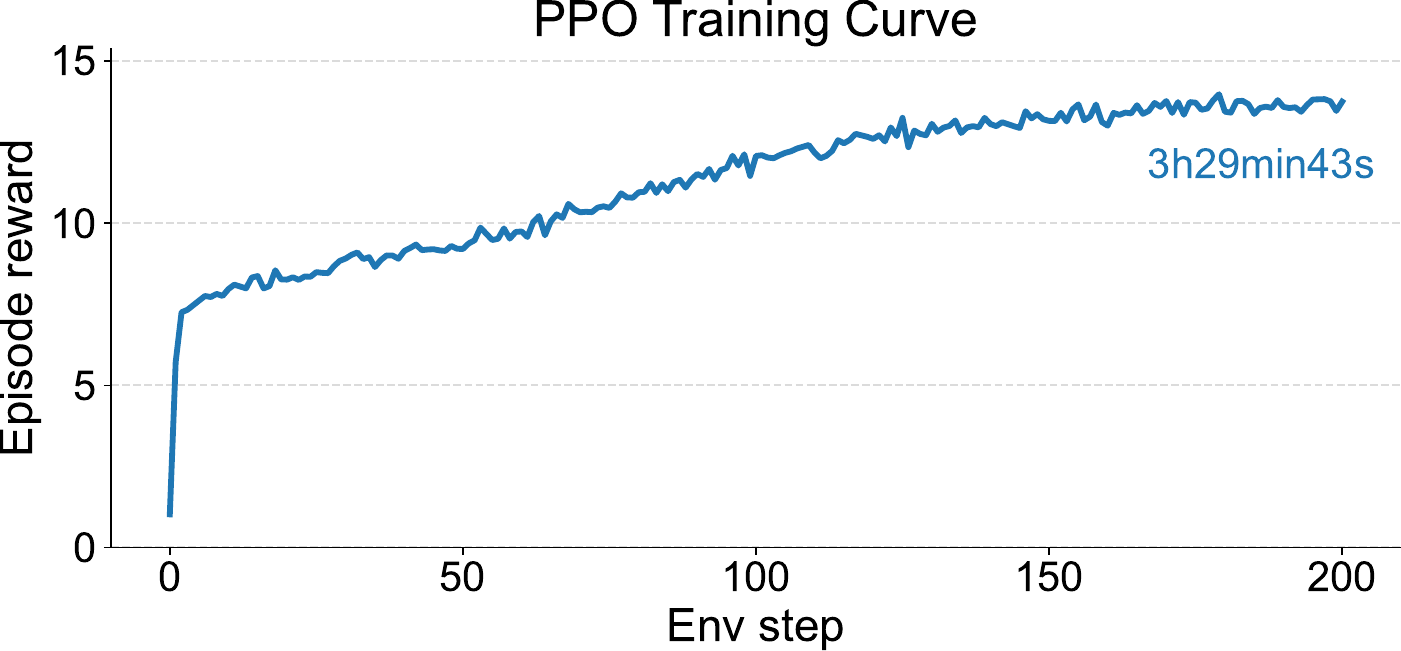}
    \caption{Mean reward curve during training of the high-level navigation policy.}
    \label{fig:nav_reward}
\end{figure}

\smallskip
\noindent\textbf{Domain Randomization.}
To improve sim-to-real transfer, we apply domain randomization during training: \textbf{initial state}---the robot's initial position and yaw are randomly sampled within the feasible area, and the target cone position is randomized around predefined anchor points with additive noise; \textbf{visual}---random perturbations to camera extrinsics, and injection of image noise and motion blur; \textbf{physical}---random external pushes on the robot base and randomized link masses.

\smallskip
\noindent\textbf{Training Hyperparameters.}
All experiments are run on a workstation with a single NVIDIA RTX 4090 GPU. We use \method with 1024 parallel environments and train the high-level navigation policy with PPO for 200 iterations. The learning rate follows an adaptive schedule with initial value $1.0 \times 10^{-3}$, and the discount factor is $\gamma = 0.98$. Further PPO and environment settings are consistent with the locomotion task where applicable.

\section{MJCF Compatibility}
\label{app:mjcf}

MJCF is a widely used format in the field of robotics simulation. \method provides extensive compatibility support for MJCF while maintaining its own simulation capabilities and features.

The details of current MJCF support status in \method are listed below:

\subsection{Global Configuration}
\method fully supports critical global options such as \texttt{timestep}, \texttt{gravity}, and solver parameters (\texttt{tolerance}, \texttt{iterations}). Contact parameters including \texttt{o\_margin}, \texttt{o\_solref}, \texttt{o\_solimp}, and \texttt{o\_friction} are also supported, ensuring consistent physics behavior. We are planning to support additional environmental factors like wind and magnetic fields in future updates.

For the compiler configuration, essential attributes like \texttt{autolimits}, \texttt{angle}, \texttt{eulerseq}, and asset directories (\texttt{meshdir}, \texttt{texturedir}) are supported, allowing for seamless model compilation.

\subsection{Asset Management}
\method supports a wide range of asset definitions:
\begin{itemize}
    \item \textbf{Mesh}: Supports \texttt{.stl}, \texttt{.obj}, and \texttt{.dae} formats. Key attributes like \texttt{file}, \texttt{vertex}, \texttt{scale}, and \texttt{refpos} are supported.
    \item \textbf{Texture \& Material}: Supports \texttt{2d} and \texttt{skybox} texture types, along with material properties such as \texttt{reflectance}, \texttt{metallic}, and \texttt{roughness} for realistic rendering.
    \item \textbf{Height Field}: Supports \texttt{hfield} definitions for complex terrain generation.
\end{itemize}

\subsection{Scene Description}
The core scene elements are well-supported to reconstruct complex robotic environments:
\begin{itemize}
    \item \textbf{Bodies \& Joints}: Supports \texttt{body} definitions with \texttt{pos}, \texttt{orientation}, and \texttt{inertial} properties. A comprehensive set of joint attributes is implemented, including \texttt{stiffness}, \texttt{damping}, \texttt{frictionloss}, \texttt{armature}, and \texttt{limited} ranges.
    \item \textbf{Geometries}: Supports primitive types (\texttt{plane}, \texttt{sphere}, \texttt{capsule}, \texttt{cylinder}, \texttt{box}) and \texttt{mesh} geoms. Contact dynamics properties like \texttt{solref}, \texttt{solimp}, \texttt{friction}, and \texttt{condim} are fully compatible.
    \item \textbf{Lights \& Cameras}: Supports \texttt{spot}, \texttt{directional}, and \texttt{point} lights with shadow casting capabilities. Cameras can be configured with \texttt{fovy}, \texttt{target}, and tracking modes (\texttt{fixed}, \texttt{track}).
\end{itemize}

\subsection{Constraints and Equality}
To model complex mechanical linkages, \method supports:
\begin{itemize}
    \item \textbf{Equality Constraints}: \texttt{connect}, \texttt{weld}, and \texttt{joint} equality constraints are supported, allowing for loop closures and rigid attachments.
    \item \textbf{Tendons}: Supports \texttt{fixed} tendons with length limits, stiffness, and damping properties.
\end{itemize}

\subsection{Actuators and Sensors}
\begin{itemize}
    \item \textbf{Actuators}: Supports \texttt{motor}, \texttt{position}, \texttt{velocity}, and \texttt{general} actuators. Control limits (\texttt{ctrllimited}, \texttt{forcerange}) and gain parameters (\texttt{kp}, \texttt{kv}, \texttt{gear}) are fully implemented.
    \item \textbf{Sensors}: A rich suite of sensors is available, including \texttt{accelerometer}, \texttt{velocimeter}, \texttt{jointpos}, \texttt{jointvel}, and frame-based sensors (\texttt{framepos}, \texttt{framequat}, \texttt{framelinvel}, etc.), enabling comprehensive state observation.
\end{itemize}

\subsection{Visuals and Defaults}
\method respects \texttt{visual} settings including global fog and lighting configurations. It also supports the \texttt{default} class system, allowing users to define hierarchical default properties for \texttt{geom}, \texttt{joint}, \texttt{material}, and other elements to streamline MJCF file structure.
