# Supplementary material for: GS-Playground: A High-Throughput Photorealistic Simulator for Vision-Informed Robot Learning
Source: arXiv:2604.25459 source file (2026-08-04)
Supplement: Supplementary file 2 [file A_Physics.tex]

\section{Physics}
\label{app:physics}

\subsection{Shaking Test}

To evaluate the stability and robustness of frictional contacts under dynamic perturbations, we conducted a "Shaking Test" using a Franka Panda arm. The robot grasps objects with different geometries—a cube, a ball, and a bottle—and executes aggressive random shaking motions. Each result aggregates 30 trials per object across three geometries. We compare the success rates of retaining the object across different physics engines at two simulation time steps: $dt=0.002s$ and $dt=0.01s$.

As shown in Table \ref{tab:franka_shaking} and Figure \ref{fig:shaking_scene}, \method demonstrates superior grasping robustness. The CPU backend achieves a 100\% success rate (90/90) across all object types and time steps, attributed to our velocity-impulse formulation and strict complementarity constraints which effectively prevent numerical drift and slippage. In contrast, MuJoCo variants (Euler, Implicit, and Implicit+Noslip) struggle significantly with this task, often dropping the object due to insufficient friction retention under high accelerations. IsaacSim and Genesis show better performance but still experience failures (60/90 success). Our GPU backend also maintains high stability, validating the effectiveness of our parallel solver design.

\begin{table}[t]
    \centering
    \caption{\small \textbf{Grasping robustness under external disturbances}. Success rates for a Franka Panda holding various geometries (cube, ball, bottle) under random shaking. A trial is successful if the object is retained for the entire evaluation horizon. 
    }
    \scalebox{1}{
        \begin{tabular}{lcc}
            \toprule
            \textbf{Engine} & \textbf{dt=0.002s (success)} & \textbf{dt=0.01s (success)} \\
            \midrule
            MuJoCo (Euler) & 0/90 & 0/90 \\
            MuJoCo (Implicit) & 0/90 & 0/90 \\
            MuJoCo (Implicit+Noslip) & 4/90 & 0/90 \\
            MJWarp & 0/90 & 10/90 \\
            IsaacSim & 60/90 & 60/90 \\
            Genesis & 60/90 & 60/90 \\
            Ours (CPU) & \textbf{90/90} & \textbf{90/90} \\
            Ours (GPU) & \textbf{90/90} & \textbf{74/90} \\
            \bottomrule
        \end{tabular}
    }
    \label{tab:franka_shaking}
\end{table}

\begin{figure}[h!]
\centering
\includegraphics[width=0.5\linewidth]{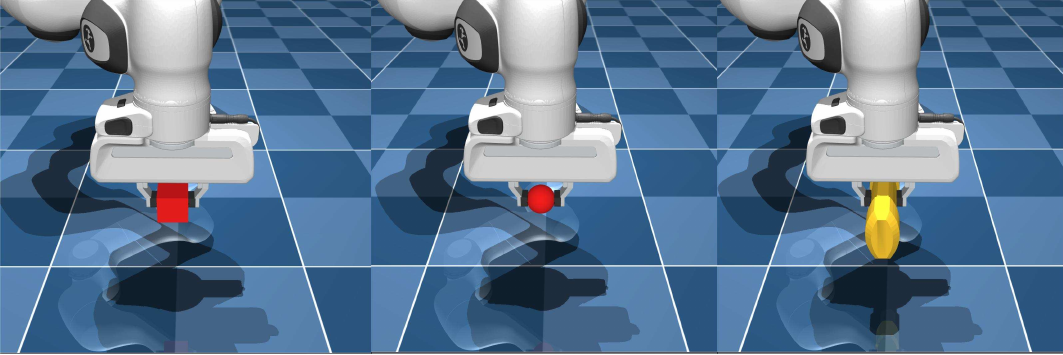}
\caption{\textbf{Shaking Test Scene}: A Franka Panda robot grasps various objects (a cube, a ball, and a bottle) while being subjected to random shaking motions. This setup is used to evaluate the grasping robustness of different simulation methods under dynamic perturbations.}
\vspace{-4mm}
\label{fig:shaking_scene}
\end{figure}

\begin{figure}[t]
    \centering
    \includegraphics[width=0.6\linewidth]{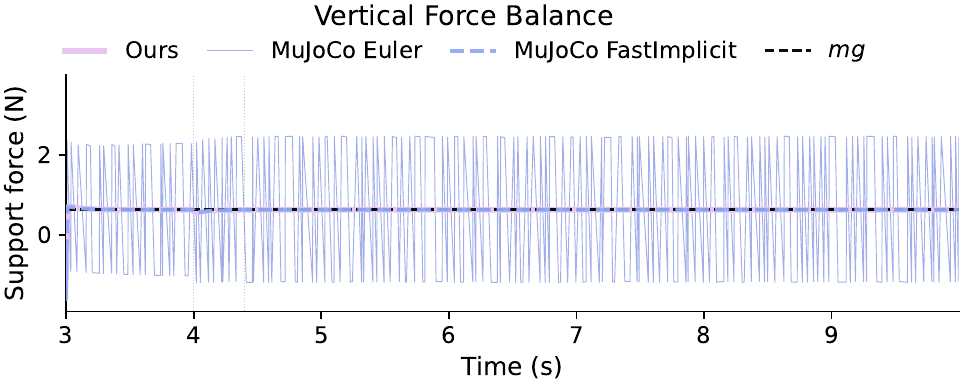}
    \caption{\textbf{Vertical force balance in a Panda grasp.}
    The plot compares the vertical contact support force $F_z$ with the theoretical object weight $mg$ during lift, settling, and hold. MuJoCo Euler exhibits large oscillatory contact forces, while \method and MuJoCo FastImplicit remain close to the force-balance target.}
    \label{fig:grasp_force_balance}
\end{figure}

\begin{table}[t]
    \centering
    \caption{\textbf{Hold-stage vertical force-balance error.}
    Mean absolute error between the measured vertical support force $F_z$ and the object weight $mg$ for the hold phase in Fig.~\ref{fig:grasp_force_balance}.}
    \label{tab:grasp_force_balance_error}
    \setlength{\tabcolsep}{5pt}
    \scalebox{0.95}{
        \begin{tabular}{lc}
            \toprule
            \textbf{Engine} & \textbf{Mean $\lvert F_z - mg \rvert$ (mN)} \\
            \midrule
            Ours & \textbf{0.039} \\
            MuJoCo FastImplicit & 0.039 \\
            MuJoCo Euler & 1740.233 \\
            \bottomrule
        \end{tabular}
    }
\end{table}

\begin{table}[t]
    \centering
    \caption{\small \textbf{Critical-friction hold test}. Each trial starts from the initialized Panda grasp hold state and runs for 5\,s with friction coefficient $\mu=\alpha\mu_{\mathrm{crit}}$. Here $\mu_{\mathrm{crit}}=mg/N=0.0902$, with $N\approx6.962$\,N and $mg=0.6278$\,N. Numeric entries report the first drop time in seconds; $\checkmark$ indicates the object remained held for the full trial. $\dagger$ marks an outcome that violates the theoretical hold/drop expectation.}
    \setlength{\tabcolsep}{3pt}
    \scalebox{0.95}{
        \begin{tabular}{lccccc}
            \toprule
            \textbf{Engine} & \textbf{0.90x} & \textbf{0.98x} & \textbf{1.00x} & \textbf{1.02x} & \textbf{1.10x} \\
            \midrule
            Theory & Drop & Drop & Hold & Hold & Hold \\
            \midrule
            \method & 0.10 & 0.25 & \textbf{$\checkmark$} & \textbf{$\checkmark$} & \textbf{$\checkmark$} \\
            MuJoCo Euler & 0.07 & 0.08 & 0.08$^\dagger$ & 0.08$^\dagger$ & 0.07$^\dagger$ \\
            MuJoCo FastImplicit & 0.10 & 0.21 & 1.23$^\dagger$ & 2.00$^\dagger$ & 2.70$^\dagger$ \\
            \bottomrule
        \end{tabular}
    }
    \label{tab:critical_friction_hold}
\end{table}

\subsection{Quantitative Grasp Force Stability}
\label{app:quantitative_grasp_force_stability}

\begin{figure}
    \centering
    \includegraphics[width=0.5\linewidth]{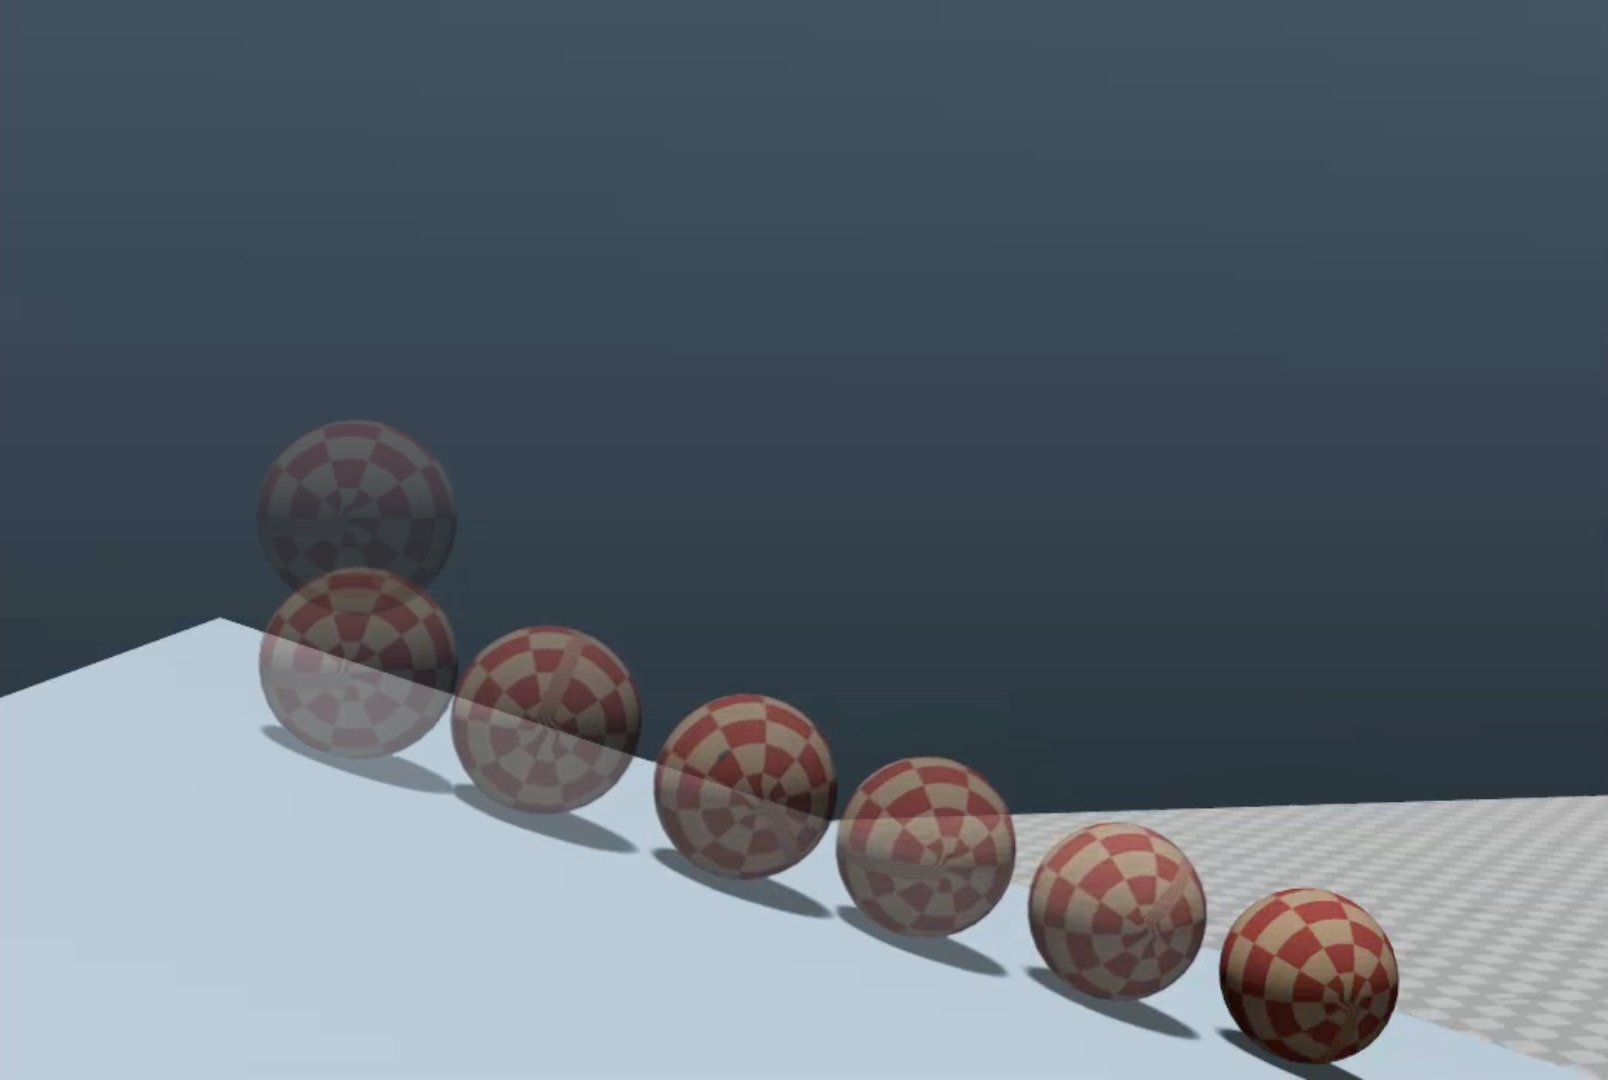}
    \caption{\textbf{Ball falling Scene:} A ball falls onto the inclined plane.}
    \label{fig:ball_falling_scene}
\end{figure}

\begin{figure}[t]
    \centering
    \includegraphics[width=0.5\linewidth]{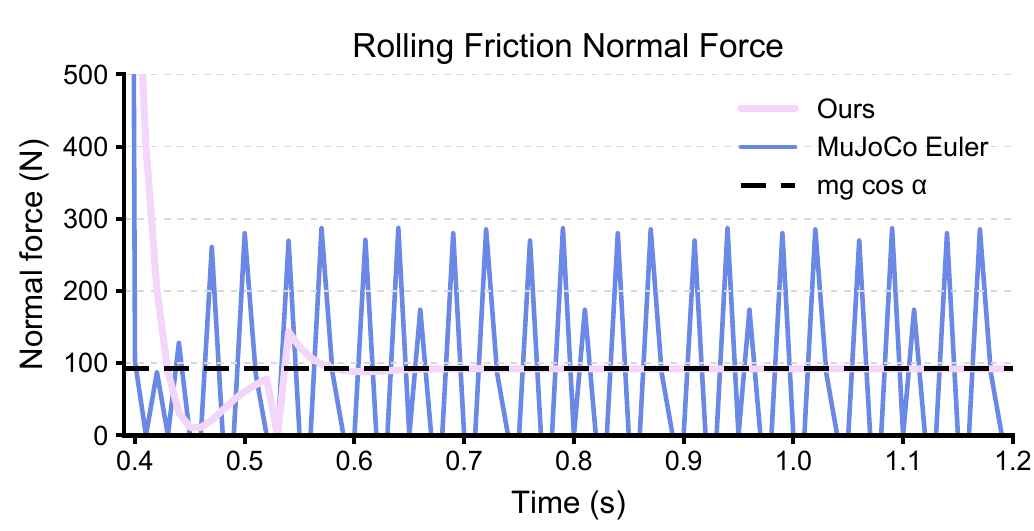}
    \caption{\textbf{Rolling friction normal force.}
    This diagram compares the normal force acting on the small ball after it contacts the inclined plane.}
    \label{fig:rolling_friction_comparison}
\end{figure}

While the shaking test evaluates task-level robustness under dynamic disturbances, it does not isolate the contact-force behavior behind a successful grasp. We therefore further examine a quasi-static hold setting where the primary question is not whether the object is retained, but whether the simulated contact forces remain physically consistent and stable.

\noindent\textbf{Vertical force balance.}
To evaluate contact stability in a quasi-static manipulation setting, we conduct a grasp hold test with a Franka Panda gripper lifting and holding a rigid cube. The robot follows the same staged trajectory for all simulators: approaching the object, closing the gripper, lifting the cube, settling after the lift, and finally maintaining a fixed hold. We compare \method against MuJoCo Euler and MuJoCo FastImplicit under the same model, control schedule, timestep, and contact-sensor layout.

The test measures whether the finger contacts provide a physically consistent vertical support force after the object leaves the table. At each simulation step, we aggregate the tangential contact forces reported by the left and right finger sensors and extract their vertical component $F_z$. During the hold phase, the expected support force is the object's weight $mg$; therefore, a stable contact solve should keep $F_z$ close to $mg$ while avoiding high-frequency oscillations. Table~\ref{tab:grasp_force_balance_error} summarizes this condition with the hold-stage mean absolute force-balance error, reported in millinewtons.

The results show that integrator choice has a strong effect on MuJoCo's contact response. Although all methods retain the object through the final hold state, MuJoCo Euler produces pronounced oscillations in the vertical support force and high hold-stage force jitter. MuJoCo FastImplicit largely suppresses this oscillation and reaches a force-balance accuracy similar to \method. In contrast, \method achieves this stable balance in its default configuration: during the hold phase, its object-height variation is $0.045$\,mm, compared with $0.230$\,mm for MuJoCo Euler and $0.190$\,mm for MuJoCo FastImplicit. This experiment therefore isolates a contact-rich manipulation regime where stable force balance, rather than binary grasp success, is the primary measurement target.

\smallskip
\noindent\textbf{Critical-friction hold.}
We further test whether the same hold state remains stable when the sliding friction coefficient is set near the theoretical limit. After a warm-up hold phase, we estimate the total normal gripping force $N$ from the finger contact sensors and compute the critical coefficient $\mu_{\mathrm{crit}}=mg/N$. We then freeze the gripper command, set the contact friction to $\alpha\mu_{\mathrm{crit}}$, and run a 5\,s fixed-hold slip test for several multipliers $\alpha$. In this experiment, $\mu_{\mathrm{crit}}=0.0902$, $N\approx6.962$\,N, $mg=0.6278$\,N, and the object mass is $0.064$\,kg.

This threshold sweep complements the force-balance measurement above. Below the critical coefficient, all methods slip as expected. At and above the theoretical threshold, \method maintains the grasp throughout the full 5\,s test, while MuJoCo Euler still drops the object almost immediately. MuJoCo FastImplicit delays the slip substantially but does not complete the hold even at $1.10\mu_{\mathrm{crit}}$. Together, the two measurements show that the evaluated grasp is not merely successful at the task level: \method also maintains a consistent force balance and preserves the hold under near-critical friction conditions.

\subsection{Normal Force Stability in Rolling Friction}
We tested a scenario \ref{fig:ball_falling_scene} where a small ball falls onto an inclined plane, with the rolling friction coefficient slightly larger than the theoretical threshold required for it to stop. In MuJoCo, during the first few frames of contact with the inclined plane, the ball experiences a large normal force that pushes it away from the surface, causing the normal force to drop to zero. The ball then falls back onto the plane, generating another large normal force. This process repeats continuously until the ball leaves the plane. In other words, the ball keeps bouncing down the inclined plane without stopping, with the normal force shaking between $0$ and $500$\,N. In contrast, in \method, the normal force experienced by the ball on the inclined plane eventually converges stably to the theoretical value, and the ball is able to come to a stop on the plane.

The sphere is a homogeneous ball with a mass of $10$\,kg, and the angle between the inclined plane and the ground is approximately $20^\circ$. Theoretically, as long as the rolling friction coefficient is greater than $0.1823$, the sphere should be able to decelerate to a stop on the inclined plane, so we set the rolling friction coefficient to $0.183$. The normal force acting on the sphere should be $92.165$\,N.
We can see from Fig.~\ref{fig:rolling_friction_comparison} that MuJoCo exhibits high-frequency shake while \method demonstrates stable convergence.
