# Supplementary material for: GS-Playground: A High-Throughput Photorealistic Simulator for Vision-Informed Robot Learning
Source: arXiv:2604.25459 source file (2026-08-04)
Supplement: Supplementary file 3 [file B_Assets.tex]

\section{3DGS Asset and Rendering}
\label{app:assets}

\subsection{Assets Generation}
\label{app:bridge_gs}
Building upon the widely used Bridge-v2 dataset\footnote{H. Walke et al., ``BridgeData V2: A Dataset for Robot Learning at Scale,'' in \textit{Conference on Robot Learning (CoRL)}, 2023.}, we introduce the Bridge-GS dataset, a large-scale collection of simulation-ready 3D visual assets produced by our automated reconstruction pipeline. Bridge-v2 spans 24 scene categories across five object families; our pipeline has produced thousands of usable Bridge-GS scenes, with successful reconstructions for most scenes after automatic processing and filtering. Dataset-scale generation is run as an offline, parallel pipeline across multiple GPUs rather than as serial per-scene processing. While the original Bridge-v2 dataset primarily consists of RGB images and robot trajectories, Bridge-GS significantly enriches this data by providing fully reconstructed scene-level and object-level 3D Gaussian Splatting (3DGS) representations, along with object-level meshes, 6D object poses, and calibrated camera intrinsics and extrinsics.

Figure \ref{fig:gs_datasets} illustrates samples from the Bridge-GS dataset. The dataset covers diverse real-world scenes reconstructed as photorealistic 3DGS environments for robot interaction. Each column represents a distinct scene processed by our pipeline. The top row displays the original RGB images from the Bridge-v2 dataset. The subsequent rows show the intermediate and final outputs of our pipeline: the estimated depth maps used for geometry estimation, the instance segmentation masks identifying interactable objects, and the final composited 3DGS assets rendered in the simulation environment. Challenging cases include heavy occlusion or stacking, transparent or highly reflective objects, and foundation-model errors that require filtering. This rich set of 3D annotations empowers researchers to train visuomotor policies in high-fidelity simulated replicas of real-world environments.

In addition to Bridge-v2, we further validate our pipeline using the InteriorGS dataset\footnote{SpatialVerse Research Team, Manycore Tech Inc., ``InteriorGS: A 3D Gaussian Splatting Dataset of Semantically Labeled Indoor Scenes,'' 2025. \url{https://huggingface.co/datasets/spatialverse/InteriorGS}}. Although InteriorGS provides ground-truth 3DGS representations, we utilize it strictly as a source of diverse indoor RGB imagery. We render 2D snapshots from the scenes and feed them into our pipeline as raw input, without accessing the underlying 3D data. As shown in the bottom half of Figure~\ref{fig:gs_datasets}, our pipeline successfully reconstructs these complex indoor environments into simulation-ready visual assets---recovering geometry, segmentation, and 3DGS representations purely from the rendered images. This demonstrates the pipeline's robustness and its capability to generalize to a wide variety of indoor settings beyond the specific domain of Bridge-v2.

\begin{figure*}[t]
    \centering
    \begin{subfigure}{\linewidth}
        \centering
        \includegraphics[width=0.75\linewidth]{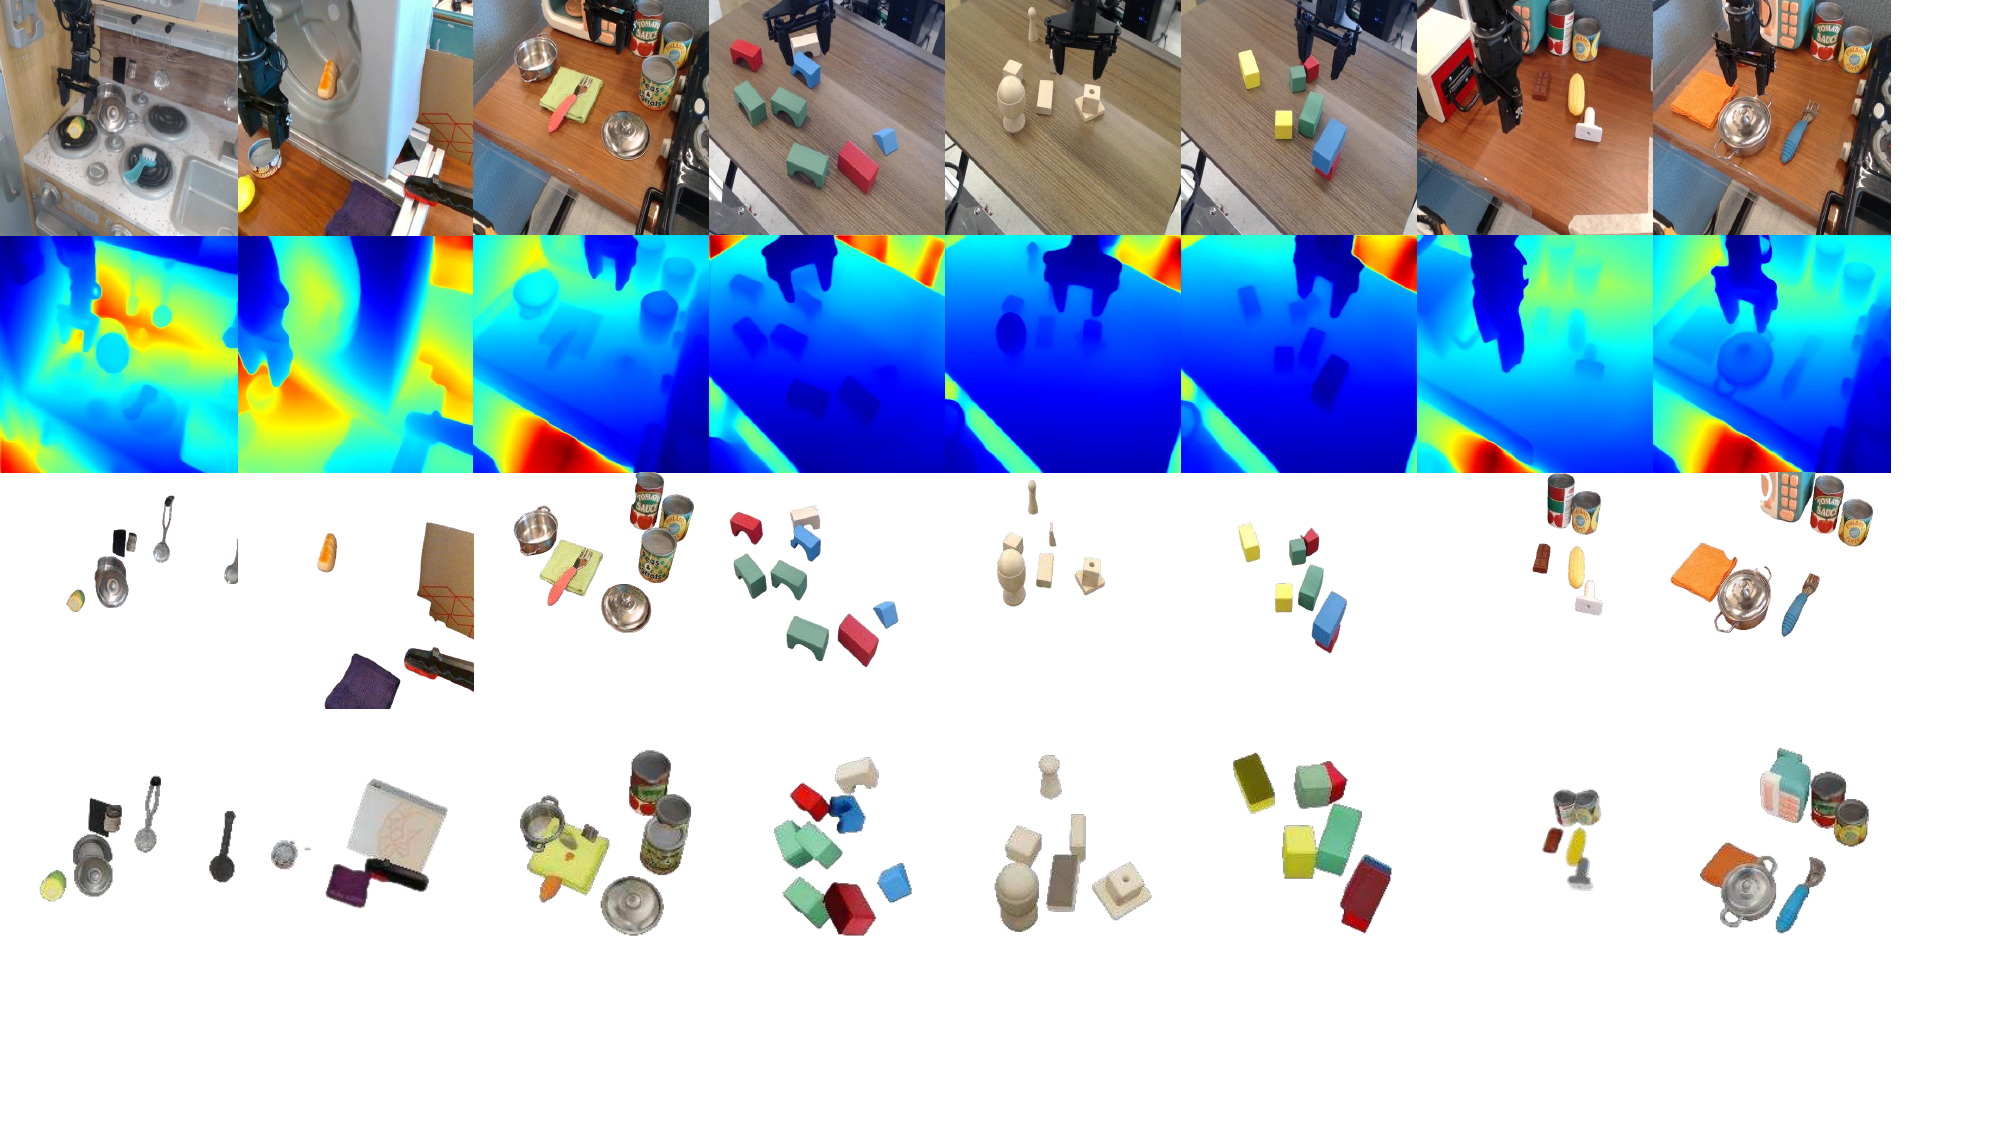}
        \label{fig:bridge_gs}
    \end{subfigure}
    \vspace{1em}
    \begin{subfigure}{\linewidth}
        \centering
        \includegraphics[width=0.75\linewidth]{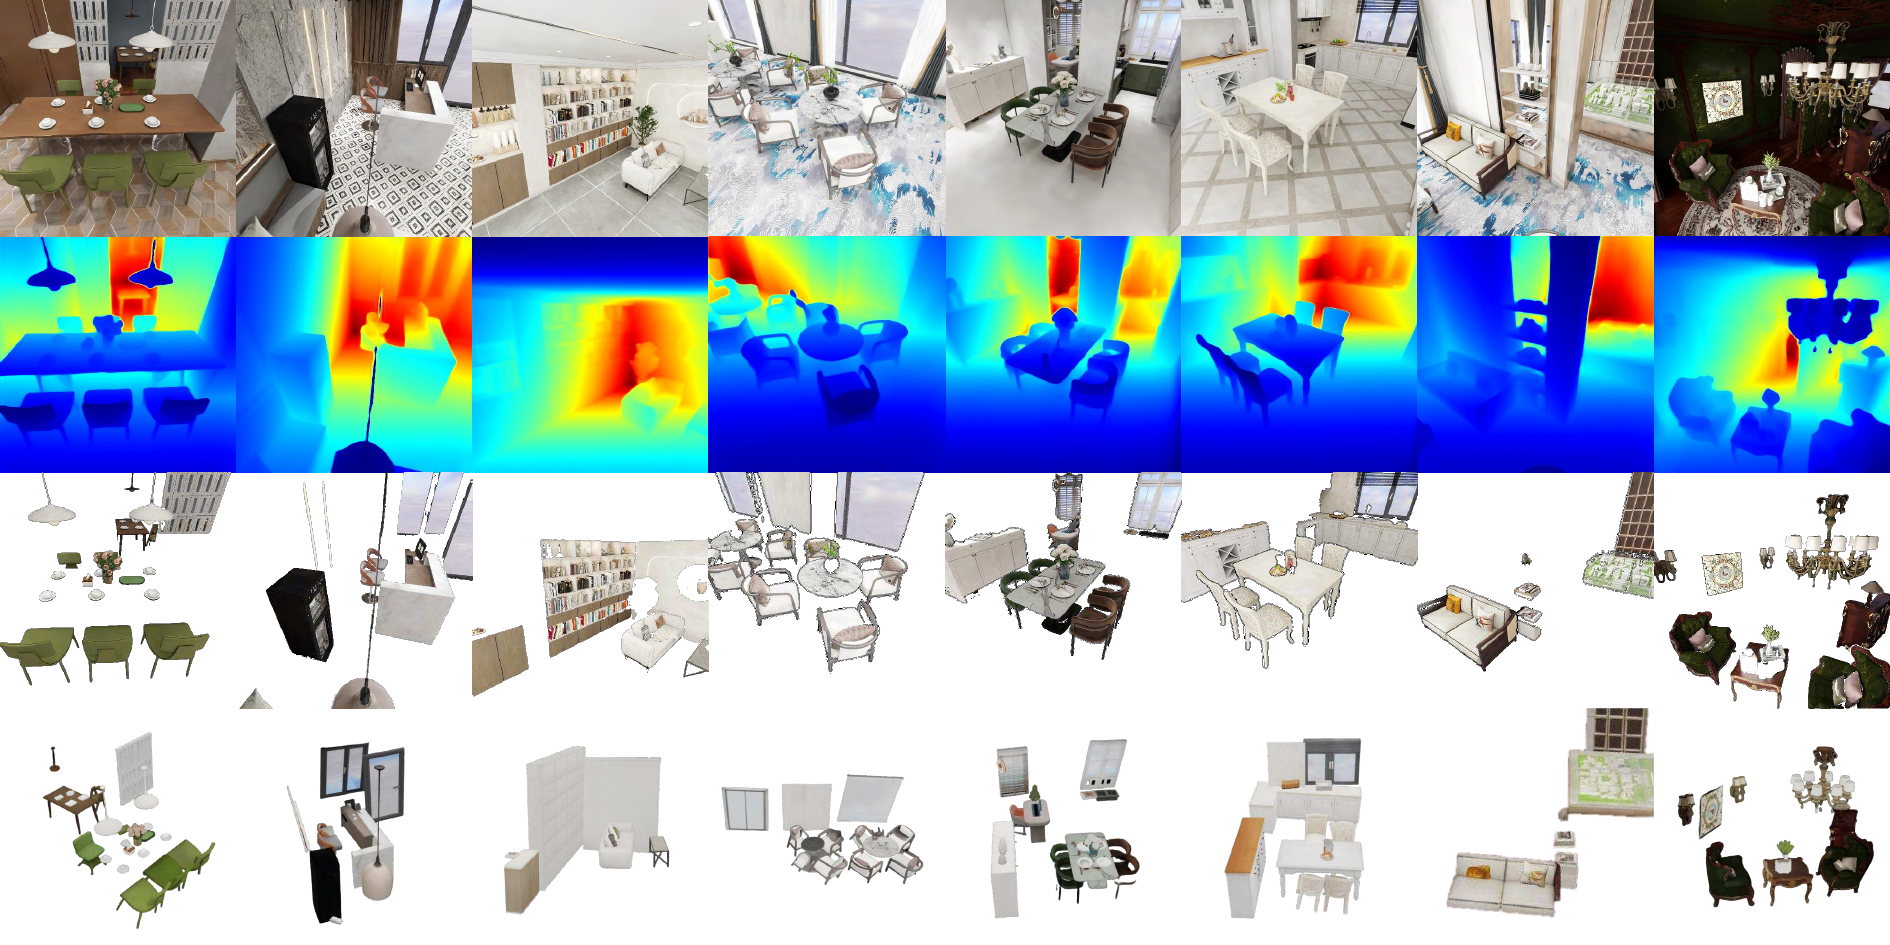}
        \label{fig:interior_gs}
    \end{subfigure}
    \caption{Visual results of the asset generation pipeline on (top) Bridge-GS and (bottom) InteriorGS datasets. The rows display: (1) Original RGB images; (2) Estimated depth maps; (3) Instance segmentation masks; and (4) Reconstructed simulation-ready 3DGS assets.}
    \label{fig:gs_datasets}
\end{figure*}

\subsection{RLGK}
\label{appendix:rlgk}
Rigid-Link Gaussian Kinematics (RLGK) is a mechanism designed to efficiently synchronize the state of millions of 3D Gaussians with the low-dimensional rigid body states derived from the physics engine. The core logic of RLGK is to map the update of high-dimensional visual representations to low-dimensional rigid body transformations, executing the synchronization process via massively parallelized vector operations on the GPU. Importantly, our implementation is optimized for \textbf{batched environments}, enabling the simultaneous simulation and rendering of $B$ parallel scenes (e.g., $B=2048$) using a single geometry template.

During the initialization phase, we upload a single "template" of the scene's Gaussians to GPU memory. We assign a rigid body index $k \in \{0, \dots, N_{bodies}\}$ to each Gaussian $g_i$ and store the initial local configuration $\{ p_{local}^i, q_{local}^i \}$ relative to the body frame.
At runtime, the physics engine outputs a batch of global poses $\mathbf{S}_t \in \mathbb{R}^{B \times N_{bodies} \times 7}$ containing the state of every rigid body in every parallel environment. RLGK performs a batched gather operation to retrieve the transform for every Gaussian across all environments simultaneously. The new global state for the $j$-th environment and $i$-th Gaussian is computed via:
\begin{align}
p_{world}^{(j,i)} &= R(q_k^{(j,t)}) p_{local}^i + t_k^{(j,t)} \\
q_{world}^{(j,i)} &= q_k^{(j,t)} \otimes q_{local}^i
\end{align}

This design allows for updating $B \times M$ points (where $M \approx 10^6$) in sub-milliseconds. By broadcasting the single template geometry $\{p_{local}^i\}$ across $B$ environments, we minimize memory bandwidth usage. The algorithmic description is provided in Algorithm \ref{alg:rlgk}.

\begin{algorithm}[h]
\centering
\caption{Batched Rigid-Link Gaussian Kinematics (RLGK)}
\label{alg:rlgk}
\begin{algorithmic}[1]
\State \textbf{Input:} Template Gaussians $\mathcal{G} = \{g_1, \dots, g_M\}$, Batch Size $B$
\State \textbf{Pre-computation:}
\For{each Gaussian $g_i \in \mathcal{G}$}
    \State Identify body index $k_i \in \{1, \dots, N_{bodies}\}$
    \State Store local pose: $p_{local}^i, q_{local}^i$
    \State $IndexMap[i] \gets k_i$
\EndFor
\State \textbf{Runtime Loop (at step $t$):}
\State Receive batch body states $\mathbf{S}_t \in \mathbb{R}^{B \times N_{bodies} \times 7}$
\State Transfer $\mathbf{S}_t$ to GPU memory
\State \textit{// Massive Parallel Update for $(B \times M)$ Gaussians}
\State $K \gets \mathbf{S}_t[:, IndexMap]$ \Comment{Gather: $(B, N_{bodies}) \to (B, M)$}
\State $\mathbf{P}_{world} \gets \text{Transform}(\mathbf{P}_{local}, K.p, K.q)$ \Comment{Broadcast $(1, M)$ to $(B, M)$}
\State $\mathbf{Q}_{world} \gets K.q \otimes \mathbf{Q}_{local}$
\State Update renderer buffers with batched state $\mathbf{P}_{world}, \mathbf{Q}_{world}$
\end{algorithmic}
\end{algorithm}

\subsection{Consistency of Policy Performance between Simulation and Real World}

\begin{figure}[h!]
    \centering
    \includegraphics[width=0.75\linewidth]{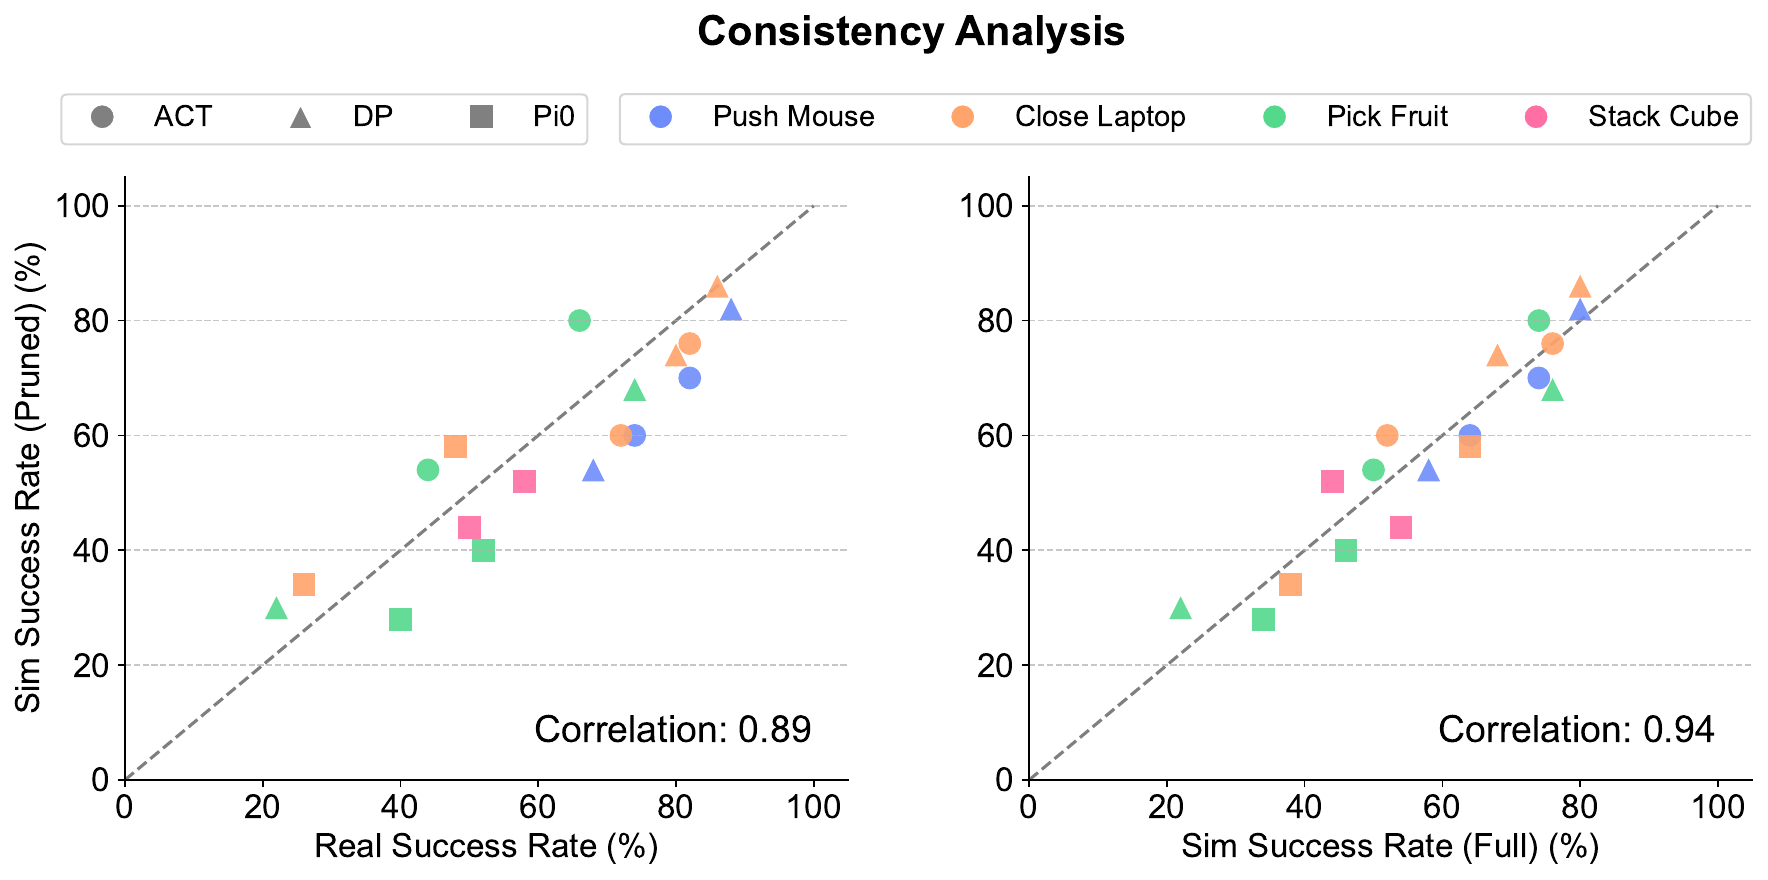}
    \caption{We compare the success rates of different policies in simulation and the real world on various tasks.}
    \label{fig:consistency_analysis}
\end{figure}

We present the consistency analysis in Figure \ref{fig:consistency_analysis}. We evaluated three representative imitation learning algorithms—ACT, Diffusion Policy (DP), and $\pi_0$—across four diverse manipulation tasks: Push Mouse, Close Laptop, Pick Fruit, and Stack Cube.
First, our experiments demonstrate a strong correlation ($0.89$) between simulation and real-world success rates, indicating good sim-real agreement across different policy architectures and task scenarios. Second, as detailed in Section \ref{sec:renderer}, our efficient pruning strategy significantly reduces the number of Gaussians while maintaining high visual fidelity. The comparison between full and pruned 3DGS rendering shows that this reduction in point count has a negligible impact on the validation success rate of imitation learning policies. This confirms that our compression strategy effectively preserves the essential visual features required for policy learning while significantly lowering the method's computational footprint.
