# Supplementary material for: GS-Playground: A High-Throughput Photorealistic Simulator for Vision-Informed Robot Learning
Source: arXiv:2604.25459 source file (2026-08-04)
Supplement: Supplementary file 4 [file C_Locomotion.tex]

\section{Locomotion}
\label{app:locomotion}

\subsection{Environment Setup}
In this task, we consider two environments: a Unitree Go2 quadruped environment and a Unitree G1 humanoid environment.

\subsection{Training Details}

\noindent\textbf{Observation and Action.}
We use a unified observation space for all environments:
\begin{itemize}
    \item Gravity projected in body frame
    \item Angular velocity
    \item Joint positions
    \item Joint velocities
    \item Previous action
    \item Velocity commands
    \item Phase
\end{itemize}
The action space is defined as absolute joint position with a default offset:
\begin{equation}
q_{t}=q_{d}+k_{a}a
\end{equation}
where $k_a$ is the action scale, $q_d$ is the default position and $a$ is the action. We employ a PD controller to map joint position to torque:
\begin{equation}
\tau =k_p(q_t-q)-k_d\dot{q}
\end{equation}

\smallskip
\noindent\textbf{Domain Randomization.}
For better sim-to-real transfer, we employ domain randomization by randomizing the following components:
\begin{itemize}
    \item \textbf{Sensor noise}: We add Gaussian noise to the data from each sensor.
    \item \textbf{Physical parameters}: Noise is introduced to physical quantities that are difficult to measure accurately, such as inertia and the center of mass, to enhance the robustness of the policy.
\end{itemize}

\smallskip
\noindent\textbf{Reward Function.}
The training rewards are detailed in Table \ref{tb:reward_design}.

\begin{table}[h]
    \centering
    \caption{Reward Functions for Locomotion Tasks} 
    \label{tb:reward_design}
    \begin{tabular}{lccc}
        \toprule
        \textbf{Reward} & \textbf{Go2 Weight} & \textbf{G1 Weight} & \textbf{Expression} \\
        \midrule
        Joint torques & -1e-5 & -1e-5& $|\tau|^2$ \\
        Dof pos limits & -1 & & $|q|-q_{max}$ \\
        Feet air time & 1 & 2 & $(t_{air}-t_{threshold})*(1-Q_{d})$ \\
        Speed tracking   & 1 & 1& $e^{-[\frac{(v_{com}-v_d)^2}{0.01}+\frac{(\omega_{com}-\omega_d)^2}{0.005}]}$ \\
        Z-axis velocity & -2 & -4 & $|v_{CoM,z}|^2$ \\
        Action rate & -0.02 & -0.01 & $|\triangle q_{last}-\triangle q|^2$ \\
        Joint acc & -2.5e-7 & -2.5e-7 & $|\frac{\dot{q}_{last}-\dot{q}}{\triangle t}|^2$ \\
        \bottomrule
    \end{tabular}
\end{table}

\smallskip
\noindent\textbf{Network Architecture.}
We employ an asymmetric actor–critic setup, in which the policy network (actor) and the value network (critic) receive different observation inputs. The policy network is fed with the aforementioned observations, while the value network additionally receives uncorrupted versions of these signals and extra sensor readings such as contact forces, perturbation forces, and linear velocity. Both policy and value networks use a three-layer multilayer perceptron (MLP) with hidden sizes of 256, 128, and 64.

\smallskip
\noindent\textbf{Training Curve.}
Learning curves for the G1 and Go2 Joystick tasks are shown in Figure~\ref{fig:g1_reward} and Figure~\ref{fig:go2_reward}, respectively.

\begin{figure}[h]
    \centering
    \includegraphics[width=0.5\linewidth]{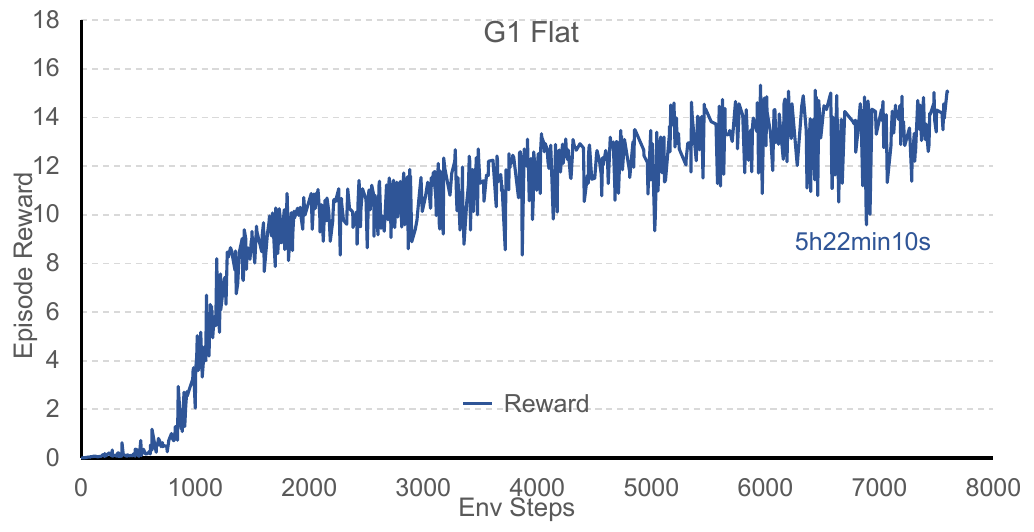}
    \caption{Learning curves for the G1 Joystick task.}
    \label{fig:g1_reward}
\end{figure}

\begin{figure}[h]
    \centering
    \includegraphics[width=0.5\linewidth]{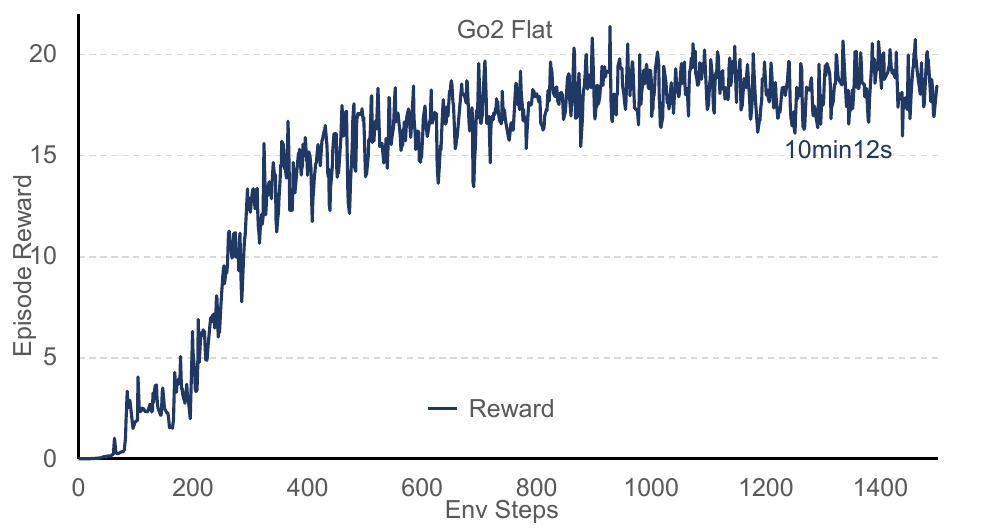}
    \caption{Learning curves for the Go2 Joystick task.}
    \label{fig:go2_reward}
\end{figure}

\subsection{Specialized Perception}
To enable robust locomotion across diverse terrains, we provide a suite of high-fidelity exteroceptive sensors compatible with various robot embodiments. As illustrated in Figure \ref{fig:loco_lidar}, these sensors can be flexibly configured to suit different tasks and morphologies.

\smallskip
\noindent\textbf{Height Scan.}
The Height Scan sensor projects a grid of ray-casts downwards around the robot base to sample terrain elevation relative to the body frame. This local height map provides high-frequency terrain geometry information, essential for traversability analysis on rough terrain. In our benchmarks, we equip the Unitree Go2 quadruped with this sensor to facilitate adaptive gait generation on uneven surfaces.

\smallskip
\noindent\textbf{LiDAR.}
The 3D LiDAR sensor performs omnidirectional or bounded ray-casting to generate a sparse point cloud of the environment. This modality is critical for obstacle detection, mapping, and navigation in cluttered spaces. We demonstrate its integration on the Unitree G1 humanoid for humanoid locomotion tasks.

Both sensors leverage our batched ray-casting engine to maintain high throughput during massive parallel training.

\begin{figure}[h]
    \centering
    \includegraphics[width=0.75\linewidth]{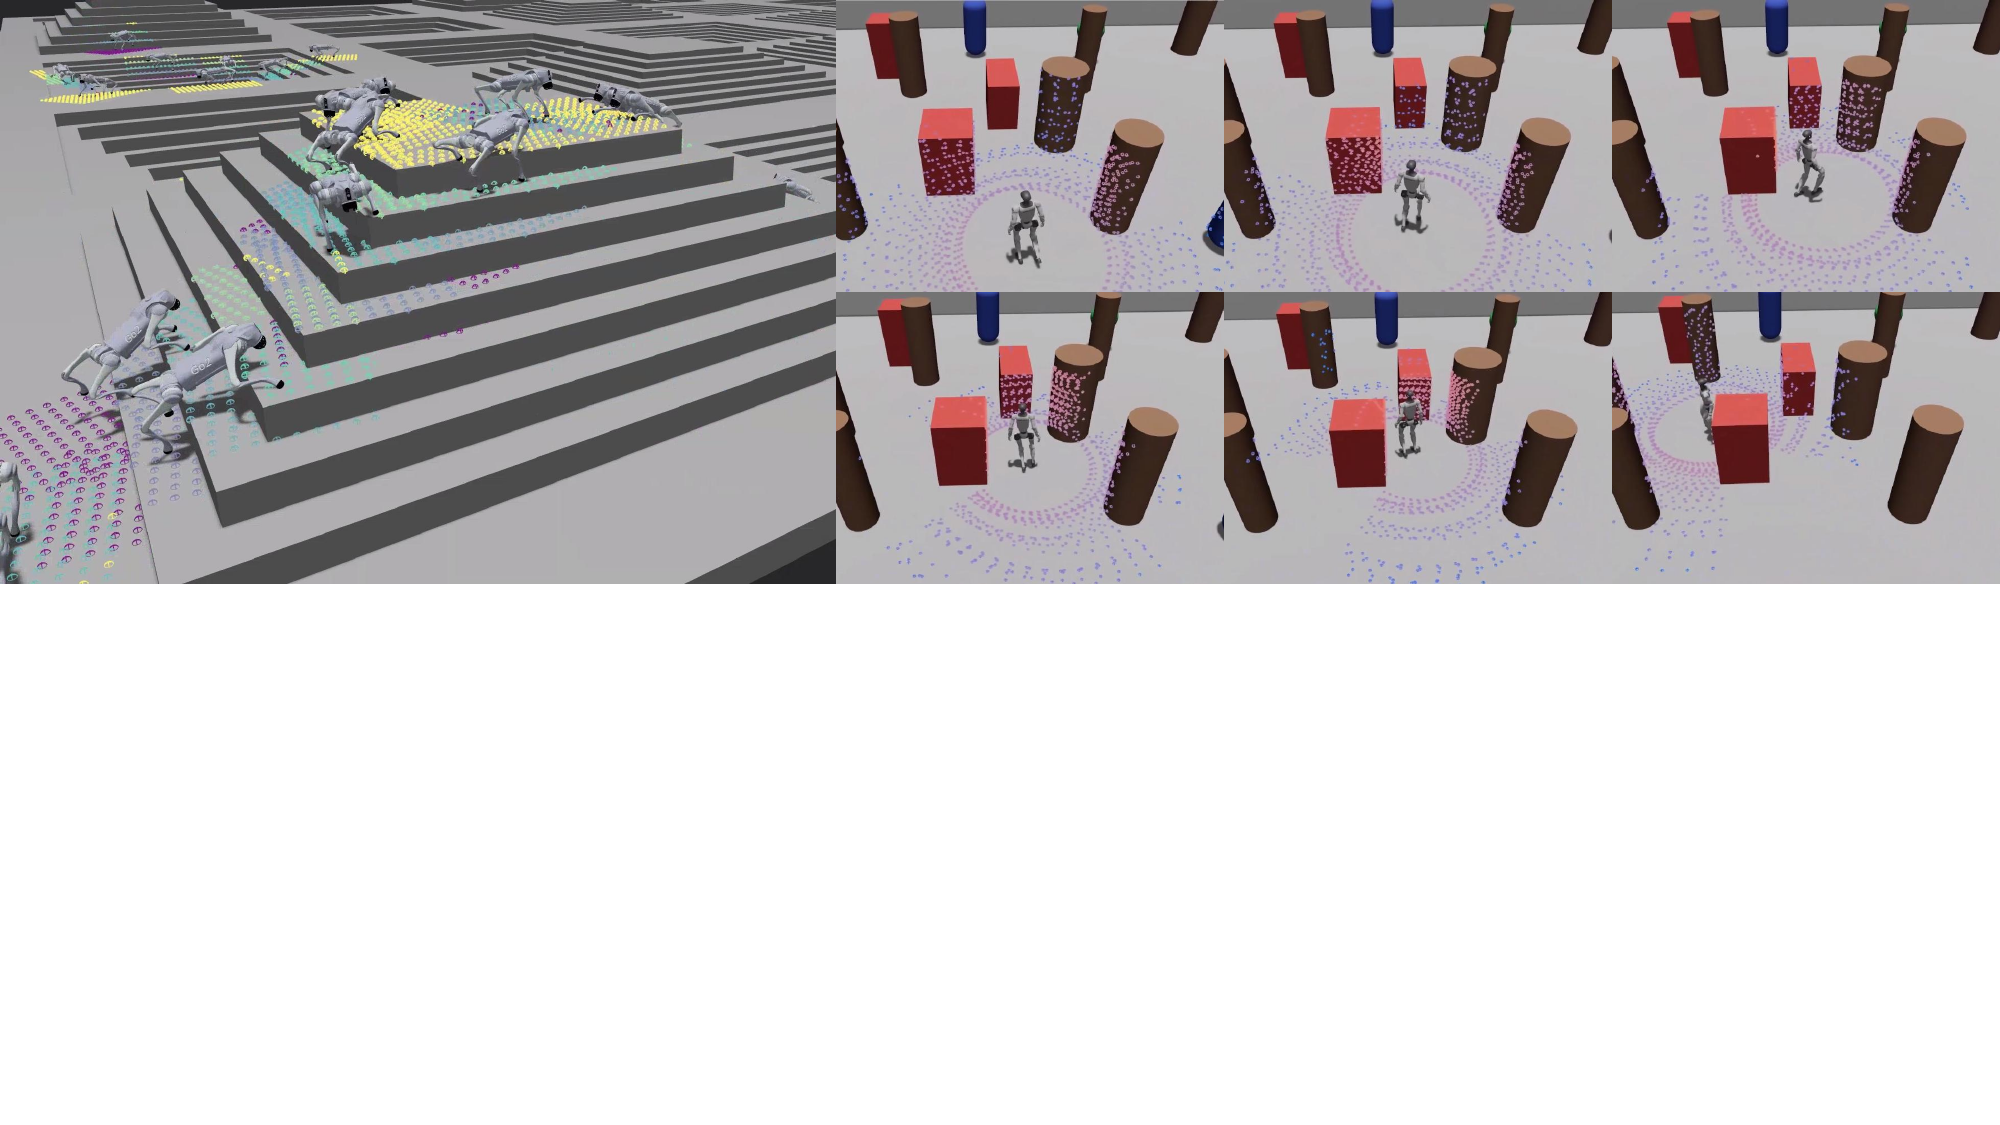}
    \caption{Perception setups for locomotion tasks. \textbf{Left:} The Unitree Go2 robot utilizing a Height Scan sensor to perceive terrain geometry on rough terrain. \textbf{Right:} The Unitree G1 humanoid equipped with a LiDAR sensor for environmental awareness.}
    \label{fig:loco_lidar}
\end{figure}
