# Supplementary material for: GS-Playground: A High-Throughput Photorealistic Simulator for Vision-Informed Robot Learning
Source: arXiv:2604.25459 source file (2026-08-04)
Supplement: Supplementary file 5 [file D_Manipulation.tex]

\section{Manipulation}
\label{app:manipulation}

\subsection{Environment Setup}
The environment used is AIRBOT Play PickCube, as shown in Figure \ref{fig:pick_cube}. The objective of this task is to control the robotic arm to grasp a cube placed on the table and lift it to a specified target position.

\begin{figure}[h]
    \centering
    \includegraphics[width=0.5\linewidth]{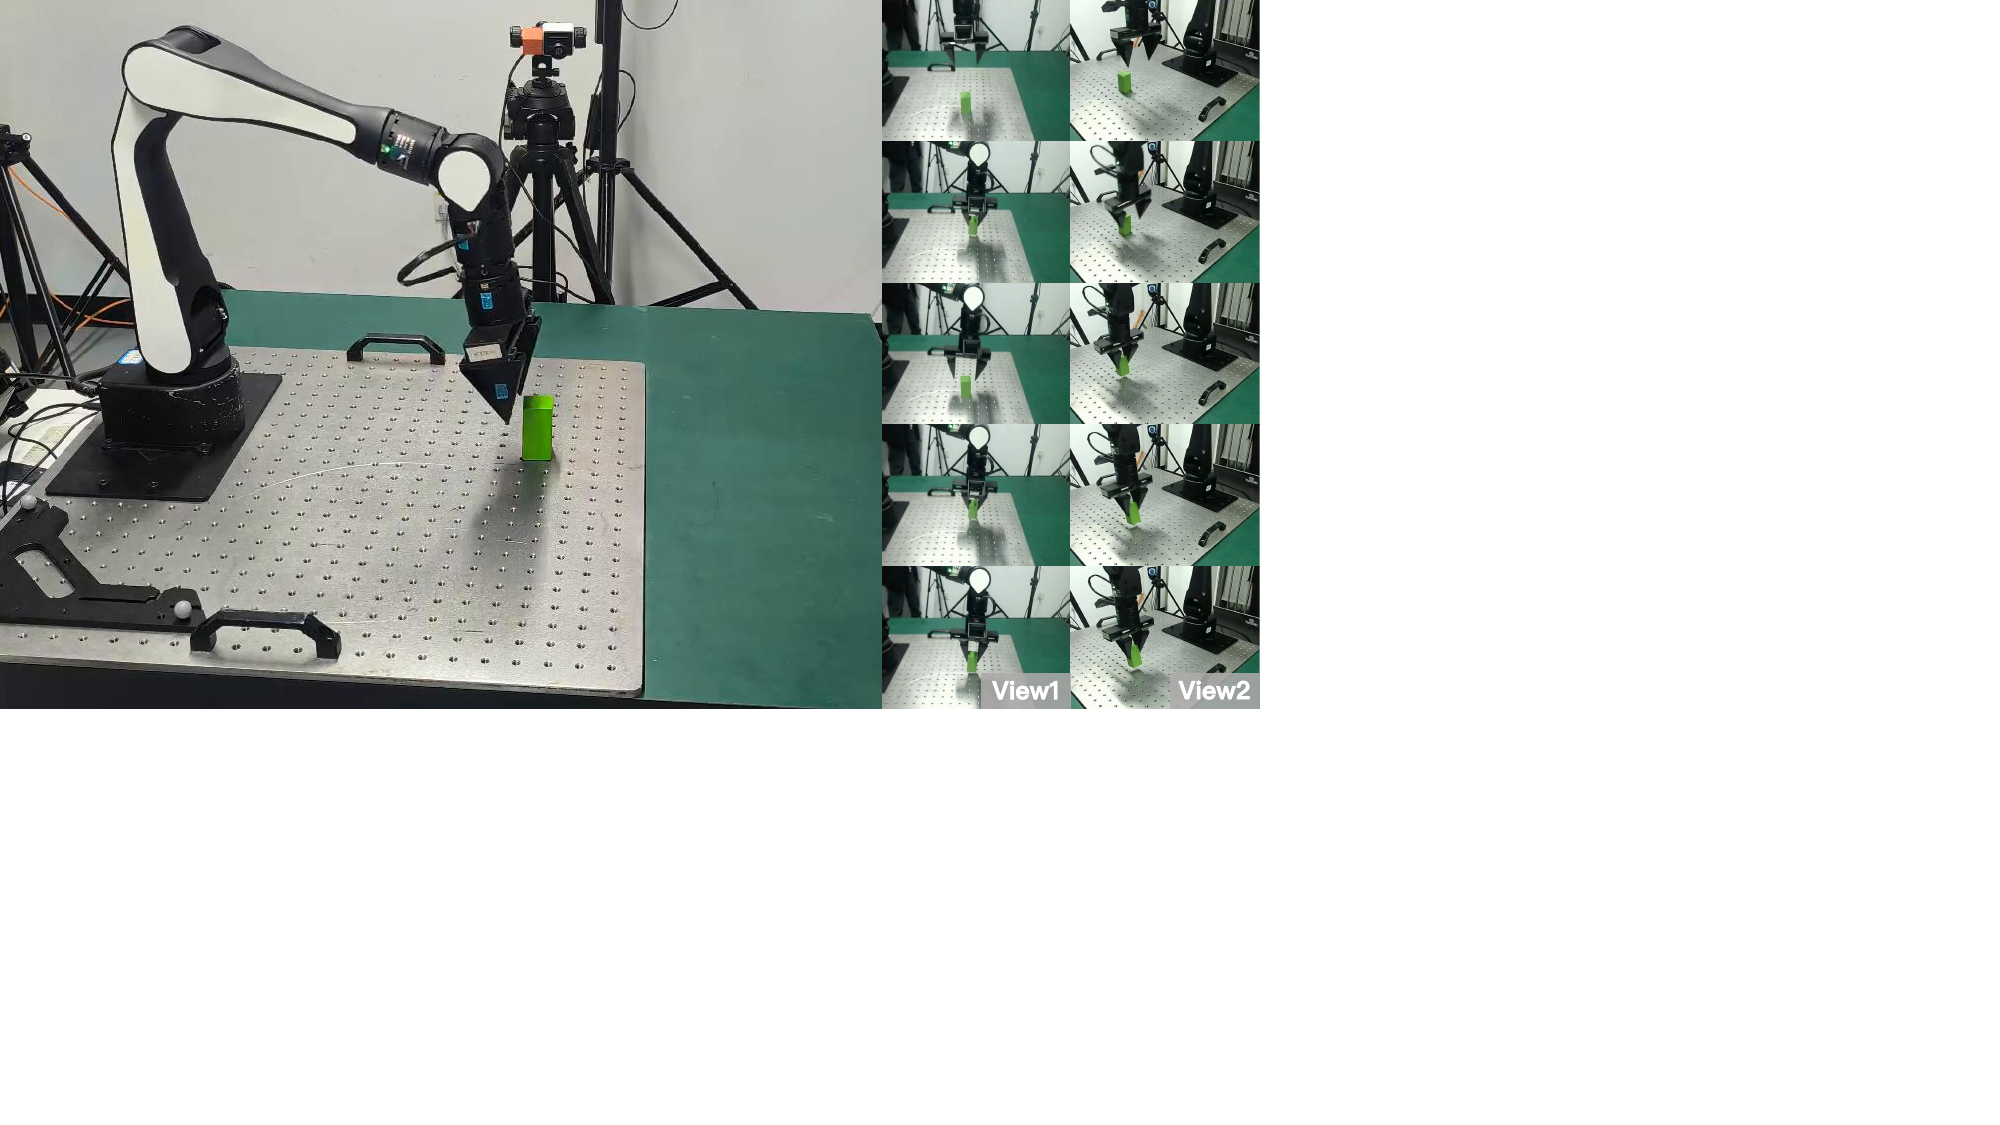}
    \caption{The AIRBOT Play PickCube manipulation environment setup. The robot needs to grasp the green cube and lift it to the target position.}
    \label{fig:pick_cube}
\end{figure}

\subsection{Training Details}

\noindent\textbf{Observation and Action.}
\begin{itemize}
    \item \textbf{Observation Space}
    \begin{itemize}
        \item Arm joint positions
        \item Gripper position
        \item Target position
        \item Joint tracking error: the difference between the current control command and the robot's current joint positions
        \item Two input RGB images
    \end{itemize}
    \item \textbf{Action Space}
    \begin{itemize}
        \item 6 DoF joint positions
        \item 1 Gripper position
    \end{itemize}
\end{itemize}

\smallskip
\noindent\textbf{Goal-Conditioned RL Setup.}
The observed \emph{target position} is the static placement goal (fixed within each episode); the block's initial 3D pose is randomized per reset (see below) and is \emph{not} observed, so grasping must rely on the two RGB streams---removing them drops zero-shot success to 0\%.

\smallskip
\noindent\textbf{Domain Randomization.}
\begin{itemize}
    \item \textbf{Camera poses}: We perform multi-camera domain randomization by perturbing each camera's extrinsics independently for every parallel world. For each camera, we add a per-axis uniform translation offset in the range $\pm0.02$ m to the nominal camera position, and apply a small random rotation by sampling a random 3D axis and a rotation angle uniformly up to $5^\circ$ (axis--angle $\to$ quaternion, then composed with the original orientation).
    \item \textbf{Box initial and target positions}: At each reset, we randomize the initial 3D positions of both the box and the target by sampling a small uniform offset around their nominal location. The box is perturbed within $\pm5$ cm in x, $\pm10$ cm in y, and 0 cm in z, while the target is perturbed within 0 cm in x, $\pm10$ cm in y, and 3--8 cm upward in z (all relative to the same nominal reference).
    \item \textbf{Image-level appearance}: We additionally apply per-environment color augmentation to rendered RGB observations, randomizing brightness, contrast, and exposure to mitigate residual photometric mismatch with the real camera (3DGS bakes static lighting; cf. Sec.~\ref{sec:limitations}).
\end{itemize}

\smallskip
\noindent\textbf{Reward Function.}

\begin{table}[h]
    \centering
    \caption{Reward Functions for PickCube Manipulation}
    \label{tab:pick_rewards}
    \begin{tabular}{@{}l c l@{}}
        \toprule
        \textbf{Reward} & \textbf{Weight} & \textbf{Expression} \\
        \midrule
        Gripper--Box Proximity & 5.0 & $1 - \tanh\!\big(5\,\lVert \mathbf{p}_{\mathrm{box}} - \mathbf{p}_{\mathrm{grip}} \rVert\big)$ \\
        Box--Target Tracking & 5.0 & $\Big(1 - \tanh\!\big(5\,\lVert \mathbf{p}_{\mathrm{tgt}} - \mathbf{p}_{\mathrm{box}} \rVert\big)\Big)\,\mathbb{I}_{\mathrm{reach}}$ \\
        No Floor Collision & 0.25 & $1 - \mathbb{I}_{\mathrm{floor}}$ \\
        No Box Collision & 0.5 & $1 - \mathbb{I}_{\mathrm{hand\text{-}box}}$ \\
        Gripper Closing & 20.0 & $\Big(1 - \frac{\lvert u_g - u_{\min} \rvert}{u_{\max}-u_{\min}}\Big)\,\mathbb{I}_{\mathrm{reach}}$ \\
        Lifted (sparse) & 8.0 & $\mathbb{I}\big(p^{z}_{\mathrm{box}} > p^{z}_{\mathrm{box,0}} + 0.005\big)\,\mathbb{I}_{\mathrm{reach}}$ \\
        Success (sparse) & 10.0 & $\mathbb{I}\big(\lVert \mathbf{p}_{\mathrm{box}} - \mathbf{p}_{\mathrm{tgt}} \rVert < \epsilon\big)$ \\
        \bottomrule
    \end{tabular}
\end{table}

\smallskip
\noindent\textbf{Notation.}
$\mathbf{p}_{\mathrm{box}}$ is the box position, $\mathbf{p}_{\mathrm{tgt}}$ is the target (mocap) position, and $\mathbf{p}_{\mathrm{grip}}$ is the gripper site position.
$p^{z}_{\mathrm{box}}$ and $p^{z}_{\mathrm{box,0}}$ denote the current and initial box height, respectively.
$u_g$ is the gripper control command (last control dimension), with limits $u_{\min}$ and $u_{\max}$.
$\mathbb{I}(\cdot)$ is the indicator function.
$\mathbb{I}_{\mathrm{reach}} = \mathbb{I}(\lVert \mathbf{p}_{\mathrm{box}} - \mathbf{p}_{\mathrm{grip}} \rVert < 0.015)$ gates rewards that should only activate after the gripper reaches the box.
$\mathbb{I}_{\mathrm{floor}}$ and $\mathbb{I}_{\mathrm{hand\text{-}box}}$ indicate floor contact and hand--box collision as detected by contact sensors.
$\epsilon$ is the success threshold (set to $0.01$ in our experiments).
The sparse bonuses "Lifted" and "Success" are applied in the vision setting.
The episode reward is computed as $\mathrm{clip}(\sum_i w_i r_i, -10^4, 10^4)$.

\smallskip
\noindent\textbf{Termination.} The episode terminates when any of the following conditions becomes true: (i) the box goes out of bounds (any coordinate exceeds 1.0 m in magnitude, or the box drops below its initial height by more than 0.01 m), (ii) the simulation state becomes non-finite (any NaN in qpos or qvel), or (iii) the task is successful.

\smallskip
\noindent\textbf{Network Architecture and Hyperparameters.}
We used the same vision PPO network as in Mujoco Playground, except that we modified the output features of the CNN encoders for both the actor and critic to 16. The training hyperparameters are shown in Table \ref{tab:ppo_hyperparameters}.

\begin{table}[h]
    \centering
    \caption{PPO Hyperparameters for Manipulation}
    \label{tab:ppo_hyperparameters}
    \begin{tabular}{lc}
        \toprule
        \textbf{Hyperparameter} & \textbf{Default Value} \\
        \midrule
        empirical\_normalization & True \\
        num\_minibatches & 8 \\
        discounting & 0.97 \\
        learning\_rate & $1\mathrm{e}{-3}$ \\
        num\_envs & 2048 \\
        num\_steps\_per\_env & 40 \\
        value\_loss\_coef & 1.0 \\
        use\_clipped\_value\_loss & True \\
        clip\_param & 0.2 \\
        entropy\_coef & 0.01 \\
        num\_learning\_epochs & 4 \\
        schedule & adaptive \\
        gamma & 0.97 \\
        lam & 0.95 \\
        desired\_kl & 0.01 \\
        max\_grad\_norm & 1.0 \\
        \bottomrule
    \end{tabular}
\end{table}

\smallskip
\noindent\textbf{Training Curve.}
In Figure~\ref{fig:pickcube_reward} we report environment steps versus reward across 4 seeds on a single A100 GPU.

\begin{figure}[h]
    \centering
    \includegraphics[width=0.5\linewidth]{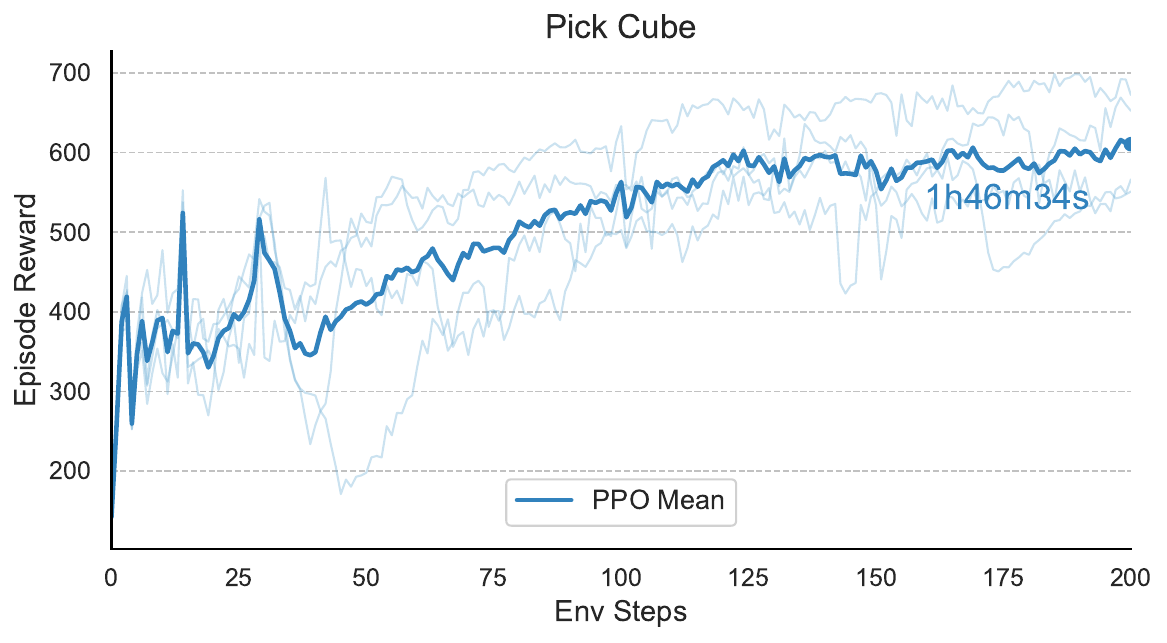}
    \caption{Learning curves for the PickCube manipulation task.}
    \label{fig:pickcube_reward}
\end{figure}
