# Supplementary material for: GS-Playground: A High-Throughput Photorealistic Simulator for Vision-Informed Robot Learning
Source: arXiv:2604.25459 source file (2026-08-04)
Supplement: Supplementary file 6 [file E_Navigation.tex]

\section{Navigation}
\label{app:navigation}

\subsection{Task Definition}
We evaluate a simplified visual goal-seeking task in \textbf{structured indoor scenes}. The Unitree Go2 robot is required to locate and approach a \textbf{red} traffic cone based on egocentric RGB observations, within a time limit of $T_{\max} = 25$ seconds. The task is successful when the Euclidean distance between the robot's base and the center of the target cone falls below a threshold $\epsilon = 0.35$ meters. The robot's initial pose and the cone position are randomized at episode start (see Domain Randomization).

\subsection{Scene Reconstruction and Rendering}
The simulation scene is captured with an RGB camera and reconstructed using the PGSR algorithm to obtain a 3D representation suitable for rendering. During training, RGB observations are rendered from the robot dog's egocentric viewpoint (camera pose and intrinsics aligned with the Go2's onboard camera) so that the policy receives first-person visual input consistent with real-world deployment.

\subsection{Training Details}
\noindent\textbf{Observation and Action Space.}
We use a hierarchical setup: a high-level navigation policy runs at 5\,Hz and outputs velocity commands; a low-level locomotion controller runs at 50\,Hz and maps commands plus proprioception to joint targets. The low-level controller is first pre-trained with PPO under domain randomization and remains frozen during navigation training.

The observation space for the high-level policy is 228-dimensional: (1)~\textbf{Visual features} (192 dimensions), i.e., image embeddings from a Vision Transformer (ViT) encoder; (2)~\textbf{Task command} (3 dimensions), a one-hot vector indicating the target color---in this simplified task only the red cone is used; (3)~\textbf{Proprioception} (33 dimensions), including base angular velocity, projected gravity, joint positions, joint velocities, and the previous action. The action space consists of 3 continuous velocity commands $\mathbf{v}_{\mathrm{cmd}} = (v_x, v_y, \omega_{\mathrm{yaw}})$, squashed by a Tanh activation and scaled to the robot's physical limits.

\noindent\textbf{Policy Architecture.}
The high-level policy uses an asymmetric Actor-Critic structure. The Actor takes the observations above and incorporates a \textbf{pre-trained ViT encoder} (frozen during navigation training) to extract features from $224 \times 224$ RGB images, followed by an LSTM to aggregate temporal information. The Critic uses the same visual and proprioceptive inputs and follows the asymmetric design described in the locomotion appendix. Both policy and value networks are optimized with PPO.

\smallskip
\noindent\textbf{Reward Function.}
The reward function is given in Table~\ref{tab:nav_rewards}. It combines a sparse success bonus for reaching the goal with dense terms for horizontal and vertical goal distance reduction, heading alignment, stopping near the goal, velocity tracking, and an action L2 penalty. 
We use the following notation for the reward terms. Let $\mathbb{I}(\cdot)$ denote the indicator function, $\mathbf{p}_{\mathrm{root},t}$ and $\mathbf{q}_{\mathrm{root},t}$ denote the robot root position and quaternion, and $R(\cdot)$ denote the corresponding rotation matrix. The head point is defined as $\mathbf{p}_{\mathrm{head},t}=\mathbf{p}_{\mathrm{root},t}+R(\mathbf{q}_{\mathrm{root},t})[0.332,0,0]^\top$, and $\mathbf{p}_{\mathrm{goal}}$ denotes the selected cone target after applying a $0.32$\,m vertical offset. We further define $d_t=\|\mathbf{p}_{\mathrm{head},t}-\mathbf{p}_{\mathrm{goal}}\|_2$, $e^z_t=|z_{\mathrm{root},t}-z_{\mathrm{goal}}|$, where $z_{\mathrm{root},t}$ and $z_{\mathrm{goal}}$ are the $z$ coordinates of $\mathbf{p}_{\mathrm{root},t}$ and $\mathbf{p}_{\mathrm{goal}}$, respectively. Finally, $\Delta\psi_t$ is the absolute wrapped yaw error between the robot heading and the goal direction, $\mathbf{v}_{\mathrm{cmd},t}=(v_x,v_y,\omega_z)$ is the velocity command, $\mathbf{v}^{xy}_{\mathrm{cmd},t}$ and $\omega^z_{\mathrm{cmd},t}$ are its planar and yaw components, $\mathbf{v}^{xy}_{\mathrm{base},t}$ and $\omega^z_{\mathrm{base},t}$ are root velocities in the base frame, and $\mathbf{a}_t$ is the high-level policy action.

\begin{table}[h]
\caption{Reward Function for High-Level Navigation Policy}
\label{tab:nav_rewards}
\centering
\begin{tabular}{llc}
\toprule
\textbf{Reward Term} & \textbf{Expression / Description} & \textbf{Weight} \\
\midrule
\multicolumn{3}{c}{\textit{Task Rewards}} \\
\midrule
Reach Goal & $\mathbb{I}(d_t < 0.35)$ & $0.5$ \\
Goal Distance & $(d_{t-1} - d_t) \cdot \mathbb{I}(d_t > 0.25)$ & $5.0$ \\
Goal Height Distance & $e^z_{t-1} - e^z_t$ & $30.0$ \\
Goal Heading & $1 - \frac{2\Delta\psi_t}{\pi} \cdot \mathbb{I}(d_t > 0.25)$ & $0.3$ \\
Stand Still at Goal & $\mathbb{I}(d_t < 0.25)/(\|\mathbf{v}_{\mathrm{cmd},t}\|_2 + 0.4)$ & $1.0$ \\
\midrule
\multicolumn{3}{c}{\textit{Tracking and Regularization}} \\
\midrule
Linear Velocity Tracking & $\exp(-\|\mathbf{v}^{xy}_{\mathrm{cmd},t} - \mathbf{v}^{xy}_{\mathrm{base},t}\|_2^2/0.5^2)$ & $0.2$ \\
Angular Velocity Tracking & $\exp(-|\omega^{z}_{\mathrm{cmd},t} - \omega^{z}_{\mathrm{base},t}|^2/0.5^2)$ & $0.2$ \\
Action L2 & $\|\mathbf{a}_t\|_2^2$ & $-0.002$ \\
\bottomrule
\end{tabular}
\end{table}

\begin{figure}[h]
    \centering
    \includegraphics[width=0.5\linewidth]{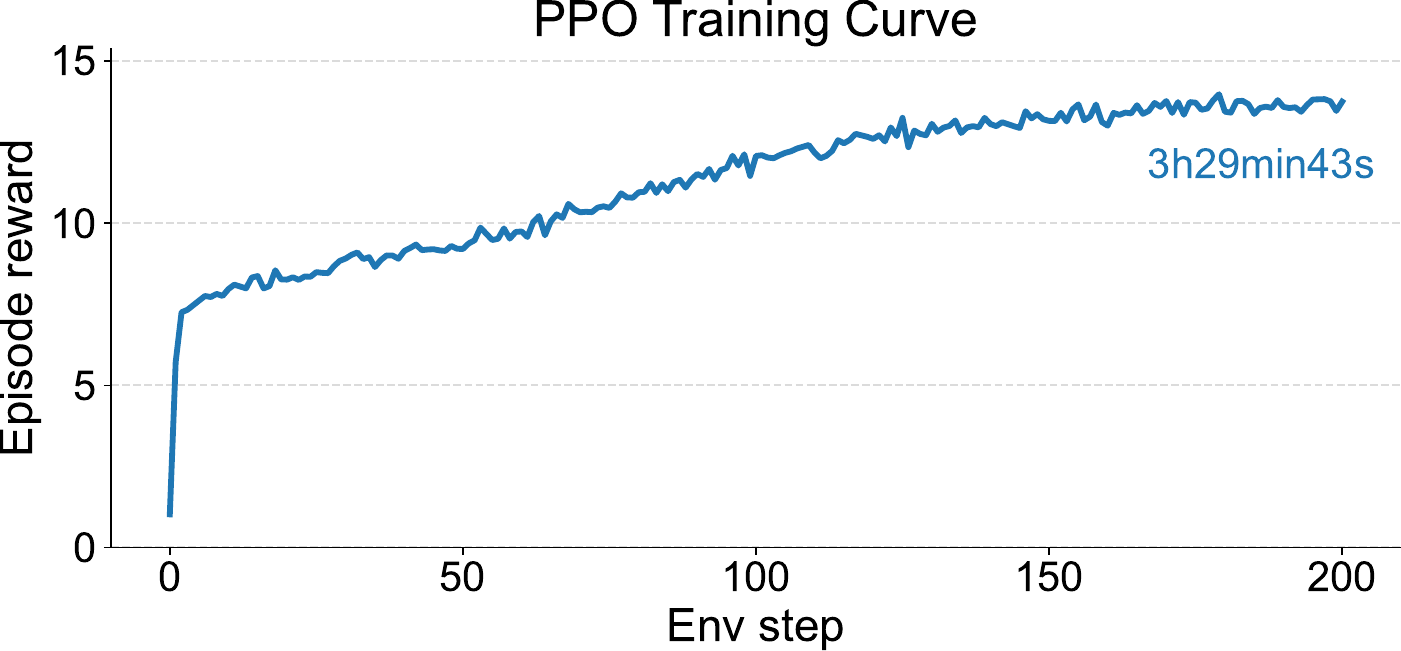}
    \caption{Mean reward curve during training of the high-level navigation policy.}
    \label{fig:nav_reward}
\end{figure}

\smallskip
\noindent\textbf{Domain Randomization.}
To improve sim-to-real transfer, we apply domain randomization during training: \textbf{initial state}---the robot's initial position and yaw are randomly sampled within the feasible area, and the target cone position is randomized around predefined anchor points with additive noise; \textbf{visual}---random perturbations to camera extrinsics, and injection of image noise and motion blur; \textbf{physical}---random external pushes on the robot base and randomized link masses.

\smallskip
\noindent\textbf{Training Hyperparameters.}
All experiments are run on a workstation with a single NVIDIA RTX 4090 GPU. We use \method with 1024 parallel environments and train the high-level navigation policy with PPO for 200 iterations. The learning rate follows an adaptive schedule with initial value $1.0 \times 10^{-3}$, and the discount factor is $\gamma = 0.98$. Further PPO and environment settings are consistent with the locomotion task where applicable.
