# Supplementary material for: GS-Playground: A High-Throughput Photorealistic Simulator for Vision-Informed Robot Learning
Source: arXiv:2604.25459 source file (2026-08-04)
Supplement: Supplementary file 7 [file F_MJCF.tex]

\section{MJCF Compatibility}
\label{app:mjcf}

MJCF is a widely used format in the field of robotics simulation. \method provides extensive compatibility support for MJCF while maintaining its own simulation capabilities and features.

The details of current MJCF support status in \method are listed below:

\subsection{Global Configuration}
\method fully supports critical global options such as \texttt{timestep}, \texttt{gravity}, and solver parameters (\texttt{tolerance}, \texttt{iterations}). Contact parameters including \texttt{o\_margin}, \texttt{o\_solref}, \texttt{o\_solimp}, and \texttt{o\_friction} are also supported, ensuring consistent physics behavior. We are planning to support additional environmental factors like wind and magnetic fields in future updates.

For the compiler configuration, essential attributes like \texttt{autolimits}, \texttt{angle}, \texttt{eulerseq}, and asset directories (\texttt{meshdir}, \texttt{texturedir}) are supported, allowing for seamless model compilation.

\subsection{Asset Management}
\method supports a wide range of asset definitions:
\begin{itemize}
    \item \textbf{Mesh}: Supports \texttt{.stl}, \texttt{.obj}, and \texttt{.dae} formats. Key attributes like \texttt{file}, \texttt{vertex}, \texttt{scale}, and \texttt{refpos} are supported.
    \item \textbf{Texture \& Material}: Supports \texttt{2d} and \texttt{skybox} texture types, along with material properties such as \texttt{reflectance}, \texttt{metallic}, and \texttt{roughness} for realistic rendering.
    \item \textbf{Height Field}: Supports \texttt{hfield} definitions for complex terrain generation.
\end{itemize}

\subsection{Scene Description}
The core scene elements are well-supported to reconstruct complex robotic environments:
\begin{itemize}
    \item \textbf{Bodies \& Joints}: Supports \texttt{body} definitions with \texttt{pos}, \texttt{orientation}, and \texttt{inertial} properties. A comprehensive set of joint attributes is implemented, including \texttt{stiffness}, \texttt{damping}, \texttt{frictionloss}, \texttt{armature}, and \texttt{limited} ranges.
    \item \textbf{Geometries}: Supports primitive types (\texttt{plane}, \texttt{sphere}, \texttt{capsule}, \texttt{cylinder}, \texttt{box}) and \texttt{mesh} geoms. Contact dynamics properties like \texttt{solref}, \texttt{solimp}, \texttt{friction}, and \texttt{condim} are fully compatible.
    \item \textbf{Lights \& Cameras}: Supports \texttt{spot}, \texttt{directional}, and \texttt{point} lights with shadow casting capabilities. Cameras can be configured with \texttt{fovy}, \texttt{target}, and tracking modes (\texttt{fixed}, \texttt{track}).
\end{itemize}

\subsection{Constraints and Equality}
To model complex mechanical linkages, \method supports:
\begin{itemize}
    \item \textbf{Equality Constraints}: \texttt{connect}, \texttt{weld}, and \texttt{joint} equality constraints are supported, allowing for loop closures and rigid attachments.
    \item \textbf{Tendons}: Supports \texttt{fixed} tendons with length limits, stiffness, and damping properties.
\end{itemize}

\subsection{Actuators and Sensors}
\begin{itemize}
    \item \textbf{Actuators}: Supports \texttt{motor}, \texttt{position}, \texttt{velocity}, and \texttt{general} actuators. Control limits (\texttt{ctrllimited}, \texttt{forcerange}) and gain parameters (\texttt{kp}, \texttt{kv}, \texttt{gear}) are fully implemented.
    \item \textbf{Sensors}: A rich suite of sensors is available, including \texttt{accelerometer}, \texttt{velocimeter}, \texttt{jointpos}, \texttt{jointvel}, and frame-based sensors (\texttt{framepos}, \texttt{framequat}, \texttt{framelinvel}, etc.), enabling comprehensive state observation.
\end{itemize}

\subsection{Visuals and Defaults}
\method respects \texttt{visual} settings including global fog and lighting configurations. It also supports the \texttt{default} class system, allowing users to define hierarchical default properties for \texttt{geom}, \texttt{joint}, \texttt{material}, and other elements to streamline MJCF file structure.
